# Supplementary material for: Beyond Born-Mayer: Improved models for short-range repulsion in ab initio force fields
Source: arXiv:1606.00734 source file (2016-06-02)
Supplement: Supplementary file 1 [file isa_ff_si.pdf]

# Supporting Information
for
'Beyond Born-Mayer: Improved models for short-range repulsion in ab initio force fields'

Mary J. Van Vleet, Alston J. Misquitta, Athony J. Stone, J.R. Schmidt

June 2, 2016

## Contents

**S1 Waldman-Hagler Analysis of $B_{ij}$ Combination Rule** **2**

**S2 Force Field Fit Quality: Exact Overlap Model vs. Slater-ISA FF** **5**

**S3 Extrapolation Algorithm for ISA Exponents** **6**

**S4 Non-polarizable, point-charge Lennard-Jones Force Fields** **8**

**S5 Born-Mayer-sISA: Scale Factor Tests** **8**
S5.1 Comparison to $S_{ij}$ . . . . . . . . 8
S5.2 Comparison to $V_{\mathrm{FF}}$ . . . . . . . . 9

**S6 Slater-OPT and Born-Mayer-OPT Force Fields** **11**

**S7 Monomer Geometries** **12**

**S8 Homomonomeric Parameters** **15**
S8.1 Multipole Moments . . . . . . . . 15
S8.2 Slater-ISA FF Parameters . . . . . . . . 18
S8.3 Born-Mayer-IP FF Parameters . . . . . . . . 21
S8.4 Born-Mayer-sISA FF Parameters . . . . . . . . 24

**S9 Force Field Fits for Homomonomeric Systems** **26**

**S10 Force Field Accuracy for LJ FF** **34**

S11Parameter Robustness for Argon 39

S12Parameter Robustness for Ethane; LJ FF results 41

# S1 Waldman-Hagler Analysis of $B_{ij}$ Combination Rule

The exact expressions for the overlap of two Slater densities $\rho_i = D_i \exp(-B_i r)$ and $\rho_j = D_j \exp(-B_j r)$ are shown here, first in the limiting case where the two exponents are equal ($B_i = B_j = B_{ij}$):

$$\begin{aligned} S^{ij}_{B_i=B_j} &= D_{ij} P(B_{ij}, r_{ij}) \exp(-B_{ij} r_{ij}) \\ D_{ij} &= \pi D_i D_j B_{ij}^{-3} \\ P(B_{ij}, r_{ij}) &= \frac{1}{3}(B_{ij} r_{ij})^2 + B_{ij} r_{ij} + 1, \end{aligned} \tag{1}$$

and second in the case where $B_i \neq B_j$:

$$\begin{aligned} S^{ij}_{B_i\neq B_j} =& \frac{16\pi D_i D_j \exp(-\{B_i + B_j\} r_{ij}/2)}{(B_i^2 - B_j^2)^3 r_{ij}} \times \\ & \Bigg[ \left(\frac{B_i - B_j}{2}\right)^2 \left( \exp\left(\{B_i - B_j\}\frac{r_{ij}}{2}\right) - \exp\left(-\{B_i - B_j\}\frac{r_{ij}}{2}\right) \right) \\ & \quad \times \left( \left(\frac{B_i + B_j}{2}\right)^2 r_{ij}^2 + (B_i + B_j) r_{ij} + 2 \right) \\ & - \left(\frac{B_i + B_j}{2}\right)^2 \exp\left(\{B_i - B_j\}\frac{r_{ij}}{2}\right) \times \left( \left(\frac{B_i - B_j}{2}\right)^2 r_{ij}^2 - (B_i - B_j) r_{ij} + 2 \right) \\ & + \left(\frac{B_i + B_j}{2}\right)^2 \exp\left(-\{B_i - B_j\}\frac{r_{ij}}{2}\right) \times \left( \left(\frac{B_i - B_j}{2}\right)^2 r_{ij}^2 + (B_i - B_j) r_{ij} + 2 \right) \Bigg]. \end{aligned} \tag{2}$$

Each overlap formula has been given a subscript to indicate limits on $B_i$ and $B_j$.

Our goal is to ascertain the extent to which $S^{ij}_{B_i\neq B_j}$ can be accurately modeled by the functional form and variables of $S^{ij}_{B_i=B_j}$. $D_i$ and $D_j$ are pre-factors appearing in both equations, and we set these variables to unity without loss of generality. To find values of $B_{ij}$ such that $S^{ij}_{B_i\neq B_j}(B_i, B_j, r_{ij}) \approx S^{ij}_{B_i=B_j}(B_{ij}, r_{ij})$, we first treat $B_{ij}$ as a completely adjustable

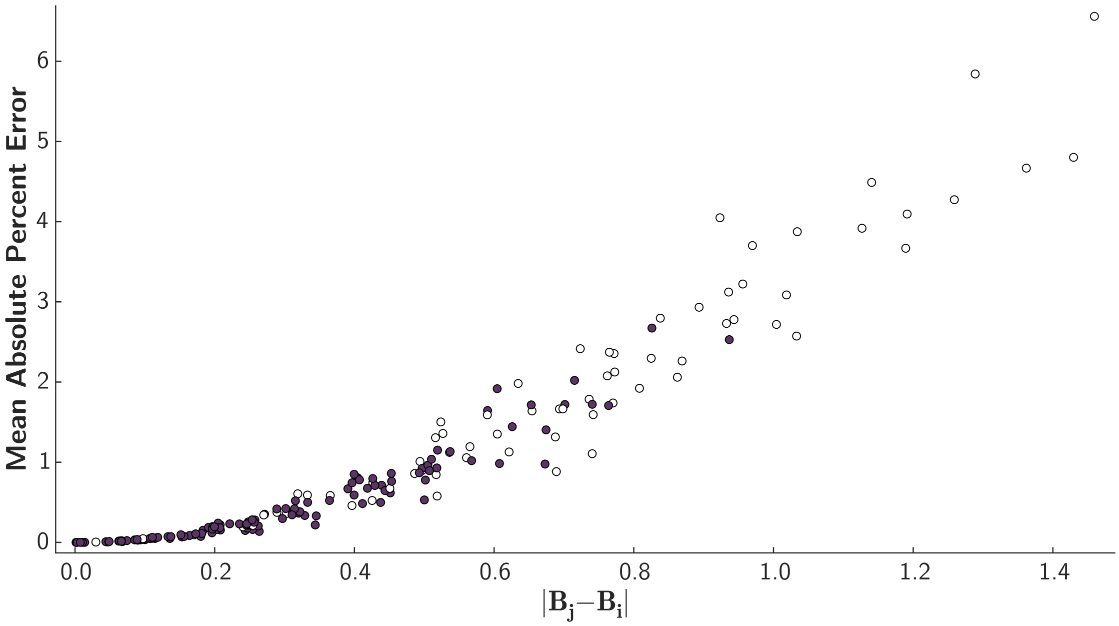


**Figure S1.** Mean absolute percent error of fitted overlap values as a function of the absolute difference between $B_i$ and $B_j$ values. Element pairs containing He, Li, Ne and/or Na are shown as empty circles. Deviations below 1% are seen for most element pairs, with noble gases and alkali metals posing a more significant challenge. Scatter in the plot is due to small variations in the absolute values of $r_{ij}$ fit for each pair. As expected, $S^{ij}_{B_i \neq B_j}$ and $S^{ij}_{B_i = B_j}$ closely agree for $|B_i - B_j| \approx 0$.

parameter, and later test for the existence of some simple combining function $f$ such that $B_{ij} = f(B_i, B_j)$.

To optimize $B_{ij}$, we first require a training set of relevant $S^{ij}_{B_i \neq B_j}$ values. $B_i$, $B_j$, and $r_{ij}$ are the only variables appearing in $S^{ij}_{B_i \neq B_j}$, and we could in principle fit $B_{ij}$ values over a grid of $B_i$, $B_j$ and $r_{ij}$ combinations. However, we are only interested in the subset of points which are chemically relevant. Consequently, we developed a library of $B_i$ values by deriving exponents from the ionization potentials of the first three rows of the periodic table (plus bromine and iodine). For each pair of elements, $B = 2\sqrt{2\mathrm{IP}}$,[1] and a range of $r_{ij}$ values corresponding to 0.8-1.2 times the sum of the van der Waals radii of the two atoms was selected. $B_{ij}$ values in $S^{ij}_{B_i = B_j}$ were then optimized (in a least-squares sense) for each element pair separately; Mean absolute percent errors (MAPE) for fitted overlaps are shown in Figure S1 and in Table S11.

Relative errors for fitting are acceptably small for all element pairs. Excluding certain noble gases and alkali metals (He, Li, Ne, Na) from consideration, these being the elements

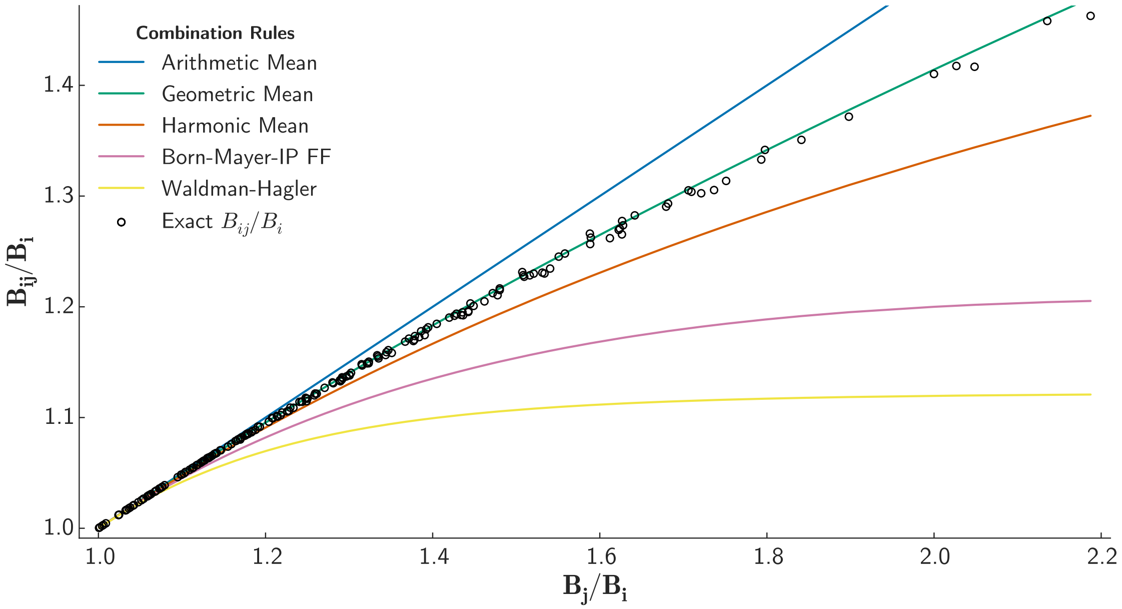


**Figure S2.** Waldman-Hagler-style analsysis of possible $B_{ij}$ combination rules. Exact $B_{ij}$ values are derived from fitting an approximate overlap density of the form $S_{ij} = A_{ij}K_2(r_{ij})\exp(-B_{ij}r_{ij})$ to the exact overlap density (as given by Rosen and by Tai[3,4]) of two distinct Slater orbitals whose exponents correspond to atomic exponents for the elements H-Ar, Cl, Br, and I. For each overlap pair, a range of $r_{ij}$ values was used from 0.8 to 1.2 times the sum of the pair's van der Waals radii. The geometric mean combination rule $B_{ij} = \sqrt{B_i B_j}$ models the exact $B_{ij}$ values with near-perfect agreement, justifying our choice of combination rule.

with the most disparate $B_i$ values compared to other elements, MAPE drops below 3% for all pairs, with the vast majority of MAPE below 1%. Our focus in this work is primarily on organic compounds where $|B_i - B_j|$ is small; empirically, these errors always translate to very small errors in the exchange energy itself. Use of an effective $B_{ij}$ may require further testing in cases with extremely disparate $B_i$ and $B_j$ values.

We next tested whether the optimized $B_{ij}$ could instead be modeled by a combination rule $B_{ij} = f(B_i, B_j)$. On the basis of symmetry and scaling considerations, Waldman and Hagler demonstrate that if a combination rule $f(B_i, B_j)$ exists, a plot of $^{B_{ij}}/_{B_i}$ vs. $^{B_j}/_{B_i}$ should lie on a single curve.[2] Remarkably (see Figure S2), a geometric mean combination rule $B_{ij} = \sqrt{B_i B_j}$ models the fitted $B_{ij}$ values with nearly quantitatively. This result allows the computation of Slater overlaps using the much simpler form of $S^{ij}_{B_i=B_j}$ (1) from individual atoms-in-molecule exponents $B_i$ and $B_j$.

# S2 Force Field Fit Quality: Exact Overlap Model vs. Slater-ISA FF

A direct test of the approximate overlap model (Equation 1 with $B_i$ values extracted from ISA calculations, synonymous with the Slater-ISA FF in the main text) is made by directly comparing the accuracy of force fields fit by the exact and approximate overlap models. Table S1 shows average RMS errors for each energy component that uses an explicit short-range term. Differences in RMS errors between models are negligible, with use of the more approximate overlap model introducing (at most) an additional 2% extra error compared to the exact overlap model. Use of $S^{ij}_{B_i=B_j}$ to compute all overlaps is thus well justified.

**Table S1.** Comparison of geometric mean RMS errors over the 91 dimer test set for the Approximate Overlap Model (that is, the Slater-ISA FF) and the Exact Overlap Model. 'Attractive' RMS errors, representing the average RMS error for the subset of points whose energies are net attractive ($E_{\text{int}} < 0$), are shown in parentheses to the right of the total average RMS errors. The average ratio of RMS errors (Slater-ISA FF/ Exact Overlap Model) for each pair in the 91 dimer test set, $\alpha$ (dimensionless), is also shown. $\alpha$ values greater than 1 indicate that on average the Exact Overlap Model is more accurate compared to the Slater-ISA FF.

| Component | Slater-ISA FF (kJ mol$^{-1}$) | Exact Overlap Model (kJ mol$^{-1}$) | $\alpha$ |
|---|---|---|---|
| Exchange | 2.641 (0.686) | 2.581 (0.679) | 1.023 (1.010) |
| Electrostatics | 1.087 (0.351) | 1.083 (0.350) | 1.004 (1.003) |
| Induction | 0.251 (0.095) | 0.252 (0.095) | 0.998 (0.999) |
| $\delta^{\text{HF}}$ | 0.246 (0.068) | 0.245 (0.068) | 1.004 (1.007) |

# S3 Extrapolation Algorithm for ISA Exponents

Unphysical asymptotic charge density decays occasionally arise in the ISA procedure due to basis set incompleteness and numerical instabilities. These unphysical decays can skew optimization of $B_i^{ISA}$ parameters, and need to be corrected. Generally speaking, there exists some range of distances in the valence region that *does* exhibit the expected exponential decay; we extrapolate the decay from this intermediate region to describe the asymptotic region using the following algorithm:

1. Take the log of each atomic density (henceforth logdens) to linearize the asymptotic density.

2. Compute the $2^{\text{nd}}$ derivative of logdens. This can be done analytically, as the BS-ISA procedure outputs an analytical expression (in terms of Gaussian basis functions) for the atomic density.

3. Determine the 'intermediate region' of exponential decay by locating the largest range where the $2^{\text{nd}}$ derivative of logdens is zero to within a fixed tolerance. Here we utilize a tolerance of 0.3 a.u. (absolute cutoff) or 190% of the smallest exponent in the Gaussian basis set (relative cutoff), whichever is smaller. The latter cutoff accounts for the eventual asymptotic Gaussian-type decay dictated by the smallest $\zeta$ in the ISA basis. The endpoints of this intermediate region are denoted $r1$ and $r2$, respectively.

4. Calculate the slope $m$ and intercept $b$ for the line defined by $r1$, $r2$, and their respective values of logdens.

5. Replace all values of logdens after $r2$ with $mr + b$. The resulting atomic density is labeled in the main text as 'Asymptotically-corrected ISA densities'.

A visual of these steps is shown in Figure S3.

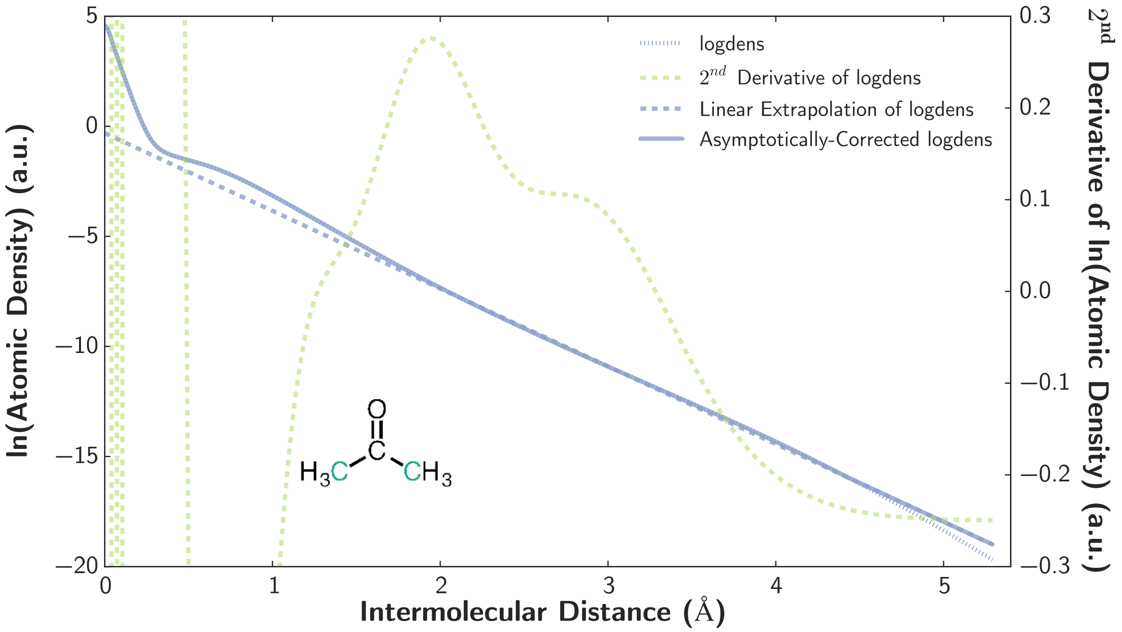


**Figure S3.** Linear extrapolation algorithm for the methyl carbon in acetone. Depicted are (in legend order) Steps 1, 2, 4, and 5 in the extrapolation algorithm. Note that some portions of the $2^{nd}$ derivative extend off the graph; also note that most of logdens is located underneath the asymptotically-corrected curve.

# S4 Non-polarizable, point-charge Lennard-Jones Force Fields

As described in the main text, a non-polarizable, rank 0 multipole version of LJ FF was fit in order to produce force fields most in line with popular standard force fields. Results for this LJ FF are shown in Table Table S2; unsurprisingly, these force fields are less accurate and less transferable compared to LJ FF in the main text, which includes polarizability and higher-order multipole moments.

**Table S2.** Comparison of characteristic RMSE and ||MSE|| over the 91 dimer test set for the non-polarizable, rank 0 multipole Lennard-Jones model. The LJ models are not parameterized on a component-by-component basis, thus RMSE/||MSE|| values for only the total FF energy is shown. 'Attractive' errors, representing the average RMSE/||MSE|| for the subset of points whose energies are net attractive ($E_{\text{int}} < 0$), are shown in parentheses to the right of the total average RMS errors. 'Dimer-Specific Fits' and 'Transferable Fits' are as in the main text.

| | Dimer-Specific Fits (kJ mol$^{-1}$) | Transferable Fits (kJ mol$^{-1}$) |
|---|---|---|
| *RMSE* | 5.116 (0.560) | 4.513 (0.658) |
| ‖*MSE*‖ | 0.803 (0.038) | 0.562 (0.079) |

# S5 Born-Mayer-sISA: Scale Factor Tests

## S5.1 Comparison to $S_{ij}$

Exact $S_{ij}$ (eq. (1) and eq. (2)) values were computed for various element pairs as in Section S1. Born-Mayer overlaps of the form

$$S_{ij} \approx K_{ij} \exp(-\xi B_{ij} r_{ij})$$

where

$$K_{ij} = \frac{K}{B_{ij}^3}$$
$$B_{ij} = \sqrt{B_i B_j}$$

were fit to these exact overlaps; $K$ and $\xi$ were optimized as universal parameters by performing a log-weighted fit over the entire set of $S_{ij}$ values.

**Table S3.** Optimized Born-Mayer parameters, $\xi$ and $K$, for fits to $S_{ij} \approx \frac{K}{(B_i B_j)^{3/2}} \exp(-\xi \sqrt{B_i B_j} r_{ij})$. $B_i$ and $B_j$ values have been chosen as in S1. Tabulated $r_{ij}$ ranges are expressed as a fraction of the sum of van der Waals radii for atoms $i$ and $j$.

| Range of $r_{ij}$ | $\xi$ | K |
|---|---|---|
| $[0.8, 1.2]$ | 0.738 | 12.2 |
| $[1.0, 2.0]$ | 0.812 | 20.9 |
| $[1.0, 4.0]$ | 0.878 | 42.6 |

Optimized parameters are shown in Table S3 for various ranges of $r_{ij}$. As shown in Table S3, the scale factor $\xi$ is highly sensitive to the values of $r_{ij}$ included in the fits, with larger values of $r_{ij}$ tending to increase $\xi$. On the other hand, $\xi$ is fairly insensitive to the values of $B_i$ and $B_j$: setting $\xi = \xi_0 + \xi_1 B_{ij}$ does not significantly improve fit quality. On the grounds of our overlap tests, it is difficult to establish a precise value for $\xi$, though our results do suggest that $\xi \sim 0.80$ and is largely independent of the atomic exponents themselves.

## S5.2 Comparison to $V_{\mathrm{FF}}$

Alternatively, we optimized the Born-Mayer-sISA FF scale factor by minimizing errors in the force field itself. Average RMS errors for a variety of scale factors are shown in Table S4. Regardless of whether we consider each energy component separately, or focus on the overall energy, setting $\xi = 0.84$ is optimal; RMS errors for this choice are comparable to the Slater-ISA FF itself.

**Table S4.** Average RMS errors over the 91 dimer test set for Born-Mayer-sISA FF using different exponential scale factors. All quantities are in kJ mol$^{-1}$ except for scale factors, which are unitless. 'Attractive' RMS errors, representing the average RMS error for the subset of points whose energies are net attractive (i.e., where $E_{tot} < 0$), are shown in parentheses to the right of the total average RMS errors. Geometric (rather than arithmetic) averages are used in all cases.

| | Born-Mayer-sISA Scale Factor | | | | | |
|---|---|---|---|---|---|---|
| Component | $\xi = 0.80$ | $\xi = 0.82$ | $\xi = 0.84$ | $\xi = 0.86$ | $\xi = 0.88$ | $\xi = 0.90$ |
| Exchange | 3.078 (0.697) | 2.690 (0.668) | 2.677 (0.686) | 2.841 (0.702) | 3.225 (0.742) | 3.798 (0.791) |
| Electrostatics | 1.144 (0.418) | 1.105 (0.378) | 1.083 (0.352) | 1.077 (0.342) | 1.104 (0.354) | 1.105 (0.373) |
| Induction | 0.258 (0.099) | 0.253 (0.097) | 0.250 (0.096) | 0.246 (0.095) | 0.243 (0.094) | 0.240 (0.094) |
| $\delta^{\mathrm{HF}}$ | 0.241 (0.072) | 0.244 (0.069) | 0.248 (0.068) | 0.255 (0.070) | 0.263 (0.075) | 0.272 (0.082) |
| Dispersion | 0.934 (0.383) | 0.803 (0.337) | 0.856 (0.336) | 1.078 (0.370) | 1.388 (0.426) | 1.740 (0.496) |
| **Total Energy** | 1.970 (0.503) | 1.775 (0.455) | 1.751 (0.453) | 1.818 (0.465) | 2.084 (0.516) | 2.451 (0.577) |

## S6 Slater-OPT and Born-Mayer-OPT Force Fields

We developed a Slater-OPT force field, identical to the Slater-ISA FF except that $B_{ij}$ parameters were optimized to reproduce the DFT-SAPT exchange-repulsion energy. Analogously, we developed Born-Mayer-OPT as an extension of the Born-Mayer-sISA FF. Treating $B_{ij}$ as a completely unconstrained parameter led to poor dispersion energies and overall transferability, and was not considered further. Instead, exponents were optimized using a harmonic penalty function of the form $k(B - B_0)^2$, with $k = 10^{-5}$ a.u. For Slater-OPT, $B_0$ values were taken from the Slater-ISA FF; for Born-Mayer-OPT, the Born-Mayer-IP FF values were used. RMS errors for Slater-OPT and Born-Mayer-OPT are shown in Table S5. For both Dimer-Specific and Transferable fits, Slater-OPT and Born-Mayer-OPT are of comparable quality. Both force fields are only slight improvements to either the Slater-ISA FF or the Born-Mayer-sISA FF; considering the extra number of free parameters required to optimize atomic exponents, we consider these results further confirmation of the inherent quality of the ISA exponents.

**Table S5.** Comparison of geometric mean RMS errors over the 91 dimer test set for the Slater-OPT and Born-Mayer-OPT methods. 'Attractive' RMS errors, representing the average RMS error for the subset of points whose energies are net attractive ($E_{\text{int}} < 0$), are shown in parentheses to the right of the total average RMS errors.

| | Dimer-Specific Fits | | Transferable Fits | |
|---|---|---|---|---|
| Component | Slater-OPT (kJ mol$^{-1}$) | Born-Mayer-OPT (kJ mol$^{-1}$) | Slater-OPT (kJ mol$^{-1}$) | Born-Mayer-OPT (kJ mol$^{-1}$) |
| Exchange | 2.513 (0.636) | 2.433 (0.639) | 2.507 (0.665) | 2.459 (0.671) |
| Electrostatics | 1.087 (0.362) | 1.068 (0.352) | 1.129 (0.359) | 1.113 (0.352) |
| Induction | 0.256 (0.097) | 0.252 (0.096) | 0.282 (0.102) | 0.280 (0.102) |
| $\delta^{\text{HF}}$ | 0.241 (0.068) | 0.244 (0.067) | 0.272 (0.077) | 0.276 (0.077) |
| Dispersion | 0.836 (0.330) | 0.822 (0.349) | 0.823 (0.331) | 0.820 (0.350) |
| **Total Energy** | | | | |
| *RMSE* | 1.549 (0.448) | 1.597 (0.450) | 1.482 (0.454) | 1.532 (0.458) |
| $\|\|MSE\|\|$ | 0.160 (0.065) | 0.160 (0.084) | 0.149 (0.057) | 0.204 (0.130) |

# S7 Monomer Geometries

Geometries for each molecule in the 91 dimer test set are listed below, in alphabetical order. Also listed are the relevant energies (highest occupied molecular orbital and ionization potential) for the asymptotic correction required in DFT-SAPT calculations of each molecule. All asymptotic corrections were performed at a PBE0/aug-cc-pVTZ level of theory. Distances and energies are in a.u.

**Table S6.** Cartesian coordinates for each molecule in the 91 dimer test set. HOMO and I.P. values, necessary for DFT-SAPT calculations, are also shown. All units are in a.u.

| **Acetone** | | | |
|---|---|---|---|
| C | 0.000000 | 0.000000 | −2.280333 |
| O | 0.000000 | 0.000000 | 0.000000 |
| C | 0.000000 | 2.435101 | −3.793814 |
| C | 0.000000 | −2.435101 | −3.793814 |
| H | 0.000000 | 4.050439 | −2.525430 |
| H | 0.000000 | −4.050439 | −2.525430 |
| H | 1.657668 | 2.514281 | −5.019869 |
| H | −1.657668 | 2.514281 | −5.019869 |
| H | −1.657668 | −2.514281 | −5.019869 |
| H | 1.657668 | −2.514281 | −5.019869 |
| HOMO: | | −0.266741 | |
| I.P.: | | 0.35386979 | |

| **Ar** | | | |
|---|---|---|---|
| Ar | 0.000000 | 0.000000 | 0.000000 |
| HOMO: | | −0.440599 | |
| I.P.: | | 0.58049447 | |

| **Chloromethane** | | | |
|---|---|---|---|
| C | 0.000000 | 0.000000 | −3.365602 |
| Cl | 0.000000 | 0.000000 | 0.000000 |
| H | 1.969851 | 0.000000 | −4.102784 |
| H | −0.984925 | 1.705856 | −4.102784 |
| H | −0.984925 | −1.705856 | −4.102784 |
| HOMO: | | −0.313074 | |
| I.P.: | | 0.41507894 | |

| **$CO_2$** | | | |
|---|---|---|---|
| C | 0.000000 | 0.000000 | 0.000000 |
| O | 0.000000 | 0.000000 | 2.196051 |
| O | 0.000000 | 0.000000 | −2.196051 |

**Table S6 – continued from previous page**

| | | | |
|---|---|---|---|
| HOMO: | | −0.394037 | |
| I.P.: | | 0.51235857 | |

**Dimethyl Ether**

| | | | |
|---|---|---|---|
| O | 0.000000 | 0.000000 | 0.000000 |
| C | 0.000000 | 2.205121 | −1.495718 |
| C | 0.000000 | −2.205121 | −1.495718 |
| H | 0.000000 | 3.871860 | −0.266451 |
| H | 0.000000 | −3.871860 | −0.266451 |
| H | 1.691305 | 2.227420 | −2.690781 |
| H | −1.691305 | 2.227420 | −2.690781 |
| H | −1.691305 | −2.227420 | −2.690781 |
| H | 1.691305 | −2.227420 | −2.690781 |
| HOMO: | | −0.272835 | |
| I.P.: | | 0.36469012 | |

**Ethane**

| | | | |
|---|---|---|---|
| C | 0.000000 | 0.000000 | 0.000000 |
| C | 0.000000 | 0.000000 | −2.902619 |
| H | −1.926009 | 0.000000 | 0.735670 |
| H | 0.963004 | 1.667872 | 0.735670 |
| H | 0.963004 | −1.667872 | 0.735670 |
| H | 1.926009 | 0.000000 | −3.638290 |
| H | −0.963004 | −1.667872 | −3.638290 |
| H | −0.963004 | 1.667872 | −3.638290 |
| HOMO: | | −0.353672 | |
| I.P.: | | 0.45125450 | |

**Ethanol**

| | | | |
|---|---|---|---|
| C | 4.487344 | −0.256436 | 0.000000 |
| C | 2.242538 | 1.511403 | 0.000000 |
| O | 0.000000 | 0.000000 | 0.000000 |
| H | −1.392728 | 1.194685 | 0.000000 |
| H | 6.208128 | 0.902911 | 0.000000 |
| H | 4.356008 | −1.440160 | 1.675998 |
| H | 4.356008 | −1.440160 | −1.675998 |
| H | 2.199641 | 2.699285 | 1.672786 |
| H | 2.199641 | 2.699285 | −1.672786 |
| HOMO: | | −0.287342 | |
| I.P.: | | 0.38582676 | |

**Ethene**

**Table S6 – continued from previous page**

| | | | |
|---|---|---|---|
| C | 0.000000 | 0.000000 | 0.000000 |
| C | 0.000000 | 0.000000 | −2.530343 |
| H | 0.000000 | 1.755367 | 1.063160 |
| H | 0.000000 | −1.755367 | 1.063160 |
| H | 0.000000 | 1.755367 | −3.593503 |
| H | 0.000000 | −1.755367 | −3.593503 |
| HOMO: | | −0.288580 | |
| I.P.: | | 0.38518748 | |

**$H_2O$**

| | | | |
|---|---|---|---|
| O | 0.000000 | 0.000000 | 0.000000 |
| H | 0.000000 | 1.430901 | −1.108324 |
| H | 0.000000 | −1.430901 | −1.108324 |
| HOMO: | | −0.333820 | |
| I.P.: | | 0.46592291 | |

**Methane**

| | | | |
|---|---|---|---|
| C | 0.000000 | 0.000000 | 0.000000 |
| H | 1.185992 | 1.185992 | 1.185992 |
| H | 1.185992 | −1.185992 | −1.185992 |
| H | −1.185992 | 1.185992 | −1.185992 |
| H | −1.185992 | −1.185992 | 1.185992 |
| HOMO: | | −0.403996 | |
| I.P.: | | 0.51955025 | |

**Methanol**

| | | | |
|---|---|---|---|
| C | 0.000000 | 2.696639 | 0.000000 |
| O | 0.000000 | 0.000000 | 0.000000 |
| H | −1.947174 | 3.401885 | 0.000000 |
| H | 0.973776 | 3.401885 | 1.686392 |
| H | 0.973776 | 3.401885 | −1.686392 |
| H | 1.709635 | −0.584303 | 0.000000 |
| HOMO: | | −0.292049 | |
| I.P.: | | 0.39901686 | |

**Methyl Amine**

| | | | |
|---|---|---|---|
| C | 0.000000 | 2.779976 | 0.000000 |
| N | 0.000000 | 0.000000 | 0.000000 |
| H | −1.887836 | 3.667203 | 0.000000 |
| H | 1.026877 | 3.452719 | 1.668817 |
| H | 1.026877 | 3.452719 | −1.668817 |
| H | −0.960170 | −0.632113 | −1.537670 |
| H | −0.960170 | −0.632113 | 1.537670 |

| Table S6 – continued from previous page | | | |
|---|---|---|---|
| HOMO: | −0.255840 | | |
| I.P.: | 0.35552078 | | |

**$NH_3$**

| | | | |
|---|---|---|---|
| N | 0.000000 | 0.000000 | 0.000000 |
| H | 0.000000 | −1.771996 | −0.721119 |
| H | 1.534647 | 0.886093 | −0.721119 |
| H | −1.534647 | 0.886093 | −0.721119 |
| HOMO: | | −0.284421 | |
| I.P.: | | 0.39987353 | |

# S8 Homomonomeric Parameters

Parameters for each molecule (as fit to homomonomeric dimers) are given for the Slater-ISA FF, the Born-Mayer-IP FF, and the Born-Mayer-sISA FF. Multipole moments are listed in the first subsection, as these values are identical for all force fields. The next subsections list $A_i$, $B_i$, $C_{i,n}$ parameters for each atom type in each molecule, as well as Drude oscillator charges $Q_{drude}$.

## S8.1 Multipole Moments

Multipole moments for each atom in each molecule are listed in Table S7. Multipoles are expressed in spherical form following notation used by Stone.[5] Note that the global coordinate system is used, with molecular geometries as in Table S6.

**Table S7.** Multipole moments for each molecule in the 91 dimer test set.

| Atomtype | $Q_{00}$ | $Q_{10}$ | $Q_{11c}$ | $Q_{11s}$ | $Q_{20}$ | $Q_{21c}$ | $Q_{21s}$ | $Q_{22c}$ | $Q_{22s}$ |
|---|---|---|---|---|---|---|---|---|---|
| **Acetone** | | | | | | | | | |
| C | 0.822823 | 0.032377 | −0.000000 | 0.000008 | 0.061201 | 0.000000 | 0.000010 | 0.069618 | −0.000000 |
| O | −0.566051 | 0.052408 | 0.000000 | −0.000006 | −0.010114 | −0.000000 | −0.000005 | 0.208541 | 0.000000 |
| C | −0.643920 | −0.019563 | 0.000000 | 0.018539 | −0.032511 | −0.000000 | 0.055572 | 0.026108 | 0.000000 |
| C | −0.643917 | −0.019574 | −0.000000 | −0.018565 | −0.032523 | −0.000000 | −0.055581 | 0.026137 | −0.000000 |
| H | 0.183107 | 0.008510 | 0.000000 | 0.005856 | 0.003477 | 0.000000 | −0.014721 | 0.007936 | −0.000000 |
| H | 0.183102 | 0.008518 | 0.000000 | −0.005869 | 0.003477 | 0.000000 | 0.014719 | 0.007935 | 0.000000 |
| H | 0.166216 | −0.003633 | 0.013504 | 0.002747 | −0.004132 | 0.004151 | 0.000390 | −0.005004 | −0.001098 |
| H | 0.166216 | −0.003633 | −0.013504 | 0.002747 | −0.004132 | −0.004151 | 0.000390 | −0.005004 | 0.001098 |
| H | 0.166211 | −0.003643 | −0.013515 | −0.002750 | −0.004130 | −0.004151 | −0.000390 | −0.005001 | −0.001097 |
| H | 0.166211 | −0.003643 | 0.013515 | −0.002750 | −0.004130 | 0.004151 | −0.000390 | −0.005001 | 0.001097 |

Table S7 – continued from previous page

| Atomtype | $Q_{00}$ | $Q_{10}$ | $Q_{11c}$ | $Q_{11s}$ | $Q_{20}$ | $Q_{21c}$ | $Q_{21s}$ | $Q_{22c}$ | $Q_{22s}$ |
|---|---|---|---|---|---|---|---|---|---|
| **Ar** | | | | | | | | | |
| Ar | −0.000001 | 0.000000 | −0.000000 | −0.000000 | 0.000000 | −0.000000 | 0.000000 | 0.000000 | −0.000000 |
| **Chloromethane** | | | | | | | | | |
| C | −0.129184 | 0.150325 | 0.000110 | −0.000000 | 0.087465 | −0.000447 | −0.000000 | 0.001151 | −0.000000 |
| Cl | −0.210641 | 0.052239 | 0.000658 | 0.000000 | 0.877399 | −0.001560 | −0.000000 | −0.001996 | 0.000000 |
| H | 0.113201 | 0.008115 | −0.002774 | 0.000000 | 0.004064 | −0.006342 | −0.000000 | 0.042912 | −0.000000 |
| H | 0.113312 | 0.008567 | 0.001173 | −0.002103 | 0.003553 | 0.003107 | −0.005492 | −0.021408 | −0.037132 |
| H | 0.113312 | 0.008567 | 0.001173 | 0.002103 | 0.003553 | 0.003106 | 0.005492 | −0.021408 | 0.037132 |
| **$CO_2$** | | | | | | | | | |
| C | 0.875432 | −0.000029 | −0.000000 | 0.000000 | 0.099260 | 0.000000 | −0.000000 | 0.000000 | −0.000000 |
| O | −0.437738 | 0.119374 | 0.000000 | −0.000000 | −0.114162 | 0.000000 | 0.000000 | −0.000000 | −0.000000 |
| O | −0.437693 | −0.119229 | 0.000000 | −0.000000 | −0.113954 | −0.000000 | 0.000000 | −0.000000 | −0.000000 |
| **Dimethyl Ether** | | | | | | | | | |
| O | −0.314909 | −0.206124 | −0.000000 | 0.000003 | −0.151378 | 0.000000 | −0.000032 | −0.276448 | 0.000000 |
| C | −0.008061 | 0.073831 | 0.000000 | −0.137375 | −0.039589 | −0.000000 | −0.120322 | −0.187908 | −0.000000 |
| C | −0.008074 | 0.073826 | 0.000000 | 0.137356 | −0.039615 | −0.000000 | 0.120322 | −0.187889 | −0.000000 |
| H | 0.081597 | 0.035961 | 0.000000 | 0.027126 | 0.012620 | −0.000000 | −0.010743 | −0.027848 | 0.000000 |
| H | 0.081596 | 0.035969 | 0.000000 | −0.027141 | 0.012620 | −0.000000 | 0.010745 | −0.027846 | −0.000000 |
| H | 0.041964 | −0.011654 | 0.038697 | −0.012289 | −0.011465 | −0.006417 | −0.031313 | −0.005419 | −0.013633 |
| H | 0.041964 | −0.011654 | −0.038697 | −0.012289 | −0.011465 | 0.006417 | −0.031313 | −0.005420 | 0.013633 |
| H | 0.041961 | −0.011665 | −0.038709 | 0.012282 | −0.011462 | 0.006414 | 0.031315 | −0.005417 | −0.013630 |
| H | 0.041961 | −0.011665 | 0.038709 | 0.012282 | −0.011462 | −0.006414 | 0.031315 | −0.005417 | 0.013630 |
| **Ethane** | | | | | | | | | |
| C | −0.252064 | −0.105205 | 0.000223 | 0.000000 | 0.017039 | 0.000023 | 0.000000 | 0.000263 | 0.000000 |
| C | −0.252073 | 0.105203 | −0.000223 | −0.000000 | 0.017046 | 0.000023 | −0.000000 | 0.000263 | 0.000000 |
| H | 0.084138 | −0.002714 | −0.029130 | 0.000000 | 0.010090 | −0.004825 | −0.000000 | 0.005963 | 0.000000 |
| H | 0.083964 | −0.002670 | 0.014633 | 0.025321 | 0.010216 | 0.002349 | 0.004123 | −0.003080 | 0.005170 |
| H | 0.083964 | −0.002670 | 0.014633 | −0.025321 | 0.010216 | 0.002349 | −0.004123 | −0.003079 | −0.005170 |
| H | 0.084139 | 0.002714 | 0.029130 | 0.000000 | 0.010090 | −0.004826 | −0.000000 | 0.005963 | −0.000000 |
| H | 0.083966 | 0.002670 | −0.014633 | −0.025321 | 0.010216 | 0.002349 | 0.004123 | −0.003079 | 0.005170 |
| H | 0.083966 | 0.002670 | −0.014633 | 0.025321 | 0.010216 | 0.002349 | −0.004123 | −0.003079 | −0.005170 |
| **Ethanol** | | | | | | | | | |
| C | −0.454684 | −0.000000 | −0.039641 | 0.014163 | −0.008827 | 0.000000 | 0.000000 | 0.010209 | −0.032164 |
| C | 0.358740 | 0.000000 | −0.069875 | −0.132865 | −0.113067 | −0.000000 | −0.000000 | 0.068791 | 0.101359 |
| O | −0.631721 | 0.000000 | 0.130683 | 0.011422 | −0.302583 | 0.000000 | −0.000000 | 0.199670 | −0.056302 |
| H | 0.378043 | 0.000000 | −0.003297 | −0.006693 | −0.026225 | 0.000000 | 0.000000 | 0.007122 | 0.007765 |
| H | 0.121728 | 0.000000 | 0.012449 | 0.016567 | −0.005502 | −0.000000 | 0.000000 | 0.003426 | 0.002573 |
| H | 0.133343 | 0.011880 | −0.013005 | −0.009345 | −0.004744 | 0.000758 | 0.003331 | 0.003627 | −0.001624 |
| H | 0.133343 | −0.011880 | −0.013005 | −0.009345 | −0.004744 | −0.000758 | −0.003331 | 0.003627 | −0.001624 |
| H | −0.019396 | 0.060093 | −0.004406 | 0.012749 | 0.002102 | −0.016691 | 0.024901 | 0.004948 | 0.006625 |
| H | −0.019396 | −0.060093 | −0.004406 | 0.012749 | 0.002102 | 0.016691 | −0.024901 | 0.004948 | 0.006625 |

Table S7 – continued from previous page

| Atomtype | $Q_{00}$ | $Q_{10}$ | $Q_{11c}$ | $Q_{11s}$ | $Q_{20}$ | $Q_{21c}$ | $Q_{21s}$ | $Q_{22c}$ | $Q_{22s}$ |
|---|---|---|---|---|---|---|---|---|---|
| **Ethene** | | | | | | | | | |
| C | −0.313293 | −0.027522 | −0.000000 | −0.000000 | −0.004502 | −0.000000 | −0.000000 | −0.032496 | −0.000000 |
| C | −0.313300 | 0.027520 | 0.000000 | 0.000000 | −0.004500 | −0.000000 | 0.000000 | −0.032493 | 0.000000 |
| H | 0.156647 | 0.006874 | 0.000000 | 0.030185 | 0.010877 | 0.000000 | −0.012146 | −0.002508 | 0.000000 |
| H | 0.156647 | 0.006874 | 0.000000 | −0.030185 | 0.010877 | 0.000000 | 0.012146 | −0.002508 | −0.000000 |
| H | 0.156649 | −0.006874 | −0.000000 | 0.030185 | 0.010877 | 0.000000 | 0.012146 | −0.002508 | −0.000000 |
| H | 0.156649 | −0.006874 | −0.000000 | −0.030185 | 0.010877 | −0.000000 | −0.012146 | −0.002508 | −0.000000 |
| **$H_2O$** | | | | | | | | | |
| O | −0.824768 | 0.164548 | −0.000000 | −0.000000 | 0.003122 | −0.000000 | 0.000000 | −0.509003 | 0.000000 |
| H | 0.412384 | 0.015330 | −0.000000 | 0.011691 | 0.007533 | −0.000000 | −0.005192 | −0.026364 | −0.000000 |
| H | 0.412384 | 0.015330 | 0.000000 | −0.011691 | 0.007533 | −0.000000 | 0.005192 | −0.026364 | −0.000000 |
| **Methane** | | | | | | | | | |
| C | −0.671142 | −0.000000 | 0.000000 | 0.000000 | 0.000000 | 0.000000 | 0.000000 | −0.000000 | 0.000000 |
| H | 0.167785 | 0.009014 | 0.009014 | 0.009014 | −0.000000 | −0.006242 | −0.006242 | −0.000000 | −0.006242 |
| H | 0.167785 | −0.009014 | 0.009014 | −0.009014 | 0.000000 | 0.006242 | −0.006242 | 0.000000 | 0.006242 |
| H | 0.167785 | −0.009014 | −0.009014 | 0.009014 | 0.000000 | −0.006242 | 0.006242 | −0.000000 | 0.006242 |
| H | 0.167785 | 0.009014 | −0.009014 | −0.009014 | −0.000000 | 0.006242 | 0.006242 | 0.000000 | −0.006242 |
| **Methanol** | | | | | | | | | |
| C | 0.018572 | 0.000000 | −0.008053 | −0.180359 | −0.134131 | −0.000000 | −0.000000 | −0.143630 | 0.003983 |
| O | −0.576407 | 0.000000 | −0.041545 | 0.164405 | −0.281268 | 0.000000 | 0.000000 | −0.044235 | −0.176494 |
| H | 0.083857 | 0.000000 | −0.047267 | 0.000587 | −0.034067 | 0.000000 | −0.000000 | −0.017460 | 0.002169 |
| H | 0.043088 | 0.042570 | 0.022329 | 0.000573 | 0.002279 | 0.019107 | −0.006061 | −0.023729 | 0.000122 |
| H | 0.043088 | −0.042570 | 0.022329 | 0.000573 | 0.002279 | −0.019107 | 0.006061 | −0.023729 | 0.000122 |
| H | 0.387801 | −0.000000 | −0.004333 | −0.003390 | −0.025935 | −0.000000 | 0.000000 | −0.015610 | −0.005664 |
| **Methyl Amine** | | | | | | | | | |
| C | 0.022408 | −0.000000 | −0.001858 | −0.174589 | −0.015557 | −0.000000 | −0.000000 | −0.132232 | 0.003031 |
| N | −0.772659 | −0.000000 | −0.030670 | 0.191476 | 0.224002 | −0.000000 | −0.000000 | −0.352581 | 0.274836 |
| H | 0.016969 | −0.000000 | −0.046914 | 0.007332 | −0.030932 | −0.000000 | −0.000000 | 0.000177 | −0.005506 |
| H | 0.059643 | 0.038600 | 0.026296 | −0.006486 | −0.006433 | 0.020931 | 0.002691 | −0.026049 | −0.000003 |
| H | 0.059643 | −0.038600 | 0.026296 | −0.006486 | −0.006433 | −0.020931 | −0.002691 | −0.026049 | −0.000003 |
| H | 0.306998 | −0.008938 | 0.012951 | 0.001795 | −0.000413 | −0.010919 | −0.012059 | −0.028898 | 0.012496 |
| H | 0.306998 | 0.008938 | 0.012951 | 0.001795 | −0.000413 | 0.010919 | 0.012059 | −0.028898 | 0.012496 |
| **$NH_3$** | | | | | | | | | |
| N | −1.050272 | 0.113155 | 0.000000 | 0.000637 | −0.661903 | 0.000000 | −0.001312 | 0.001250 | −0.000000 |
| H | 0.350420 | 0.018866 | 0.000000 | −0.007172 | −0.023309 | −0.000000 | −0.004344 | 0.015849 | 0.000000 |
| H | 0.349926 | 0.018818 | 0.006316 | 0.003662 | −0.023015 | 0.003834 | 0.002117 | −0.007862 | −0.013755 |
| H | 0.349926 | 0.018818 | −0.006316 | 0.003662 | −0.023015 | −0.003834 | 0.002117 | −0.007862 | 0.013755 |

## S8.2 Slater-ISA FF Parameters

$A_i$, $B_i$, $C_{i,n}$ parameters for the Slater-ISA FF are listed in Table S8. $A_{ij}$, $B_{ij}$, and $C_{ij,n}$ parameters can be determined from the following combination rules:

$$A_{ij} = A_i A_j$$
$$B_{ij} = \sqrt{B_i B_j}$$
$$C_{ij,n} = \sqrt{C_{i,n} C_{j,n}}$$

Parameters are given for each unique atom type in each molecule; where multiple atom types exist for a particular element, atom types are labeled first with the element name and second by connectivity. Thus the carbonyl carbon in acetone is labeled 'CO', whereas the methyl carbon is labeled 'CH'.

The total force field energy is defined by the following equations:

$$\begin{aligned}
B_i &= B_i^{ISA} \\
P(B_{ij}, r_{ij}) &= \frac{1}{3}(B_{ij} r_{ij})^2 + B_{ij} r_{ij} + 1 \\
x &= B_{ij} r_{ij} - \frac{2B_{ij}^2 r_{ij} + 3B_{ij}}{B_{ij}^2 r_{ij}^2 + 3B_{ij} r_{ij} + 3} r_{ij} \\
f_{2n}(x) &= 1 - e^{-x} \sum_{k=0}^{2n} \frac{(x)^k}{k!} \\
V_{ij}^{\text{exch}} &= A_{ij}^{exch} P(B_{ij}, r_{ij}) \exp(-B_{ij} r_{ij}) \\
V_{ij}^{\text{elst}} &= -A_{ij}^{elst} P(B_{ij}, r_{ij}) \exp(-B_{ij} r_{ij}) + \sum_{tu} Q_t^i T_{tu} Q_u^j \\
V_{ij}^{\text{ind}} &= -A_{ij}^{ind} P(B_{ij}, r_{ij}) \exp(-B_{ij} r_{ij}) + V_{\text{shell}}^{(2)} \\
V_{ij}^{\delta\text{HF}} &= -A_{ij}^{\delta\text{HF}} P(B_{ij}, r_{ij}) \exp(-B_{ij} r_{ij}) + V_{\text{shell}}^{(3-\infty)} \\
V_{ij}^{\text{disp}} &= -\sum_{n=3}^{6} f_{2n}(x) \frac{C_{ij,2n}}{r_{ij}^{2n}}
\end{aligned}$$

$$V_{\text{FF}} = \sum_{ij} V_{ij}^{\text{elst}} + V_{ij}^{\text{exch}} + V_{ij}^{\text{ind}} + V_{ij}^{\delta\text{HF}} + V_{ij}^{\text{disp}}$$

The Tang-Toennies damping function $f$ is defined in the main text; the polarization energy $V_{\text{shell}} = V_{\text{shell}}^{(2)} + V_{\text{shell}}^{(3-\infty)}$ arising from drude oscillators is defined in ref. 1.

**Table S8.** Slater-ISA FF parameters.

| Atomtype | $A_{exch}$ | $A_{elst}$ | $A_{ind}$ | $A_{\delta HF}$ | $B$ | $C_6$ | $C_8$ | $C_{10}$ | $C_{12}$ | $Q_{drude}$ |
|---|---|---|---|---|---|---|---|---|---|---|
| **Acetone** | | | | | | | | | | |
| CO | 3.804952 | 2.105976 | 2.063011 | 0.491181 | 2.604683 | 13.406 | 145.511 | 6091.546 | 80859.461 | −0.4541 |
| OC | 4.178782 | 2.590649 | 0.144518 | 1.137061 | 2.360638 | 22.881 | 353.876 | 10131.697 | 174478.272 | −0.9327 |
| CH | 2.204201 | 1.308847 | 0.000000 | 0.029237 | 1.932603 | 23.494 | 353.376 | 4001.387 | 41152.121 | −1.2947 |
| HC | 0.591374 | 0.289797 | 0.178630 | 0.223158 | 2.266776 | 2.245 | 42.098 | 1104.938 | 0.000 | 0.0000 |
| **Ar** | | | | | | | | | | |
| Ar | 6.130962 | 3.607145 | 0.816138 | 1.255571 | 2.183303 | 71.007 | 1556.382 | 37687.507 | 709695.360 | −1.0694 |
| **Chloromethane** | | | | | | | | | | |
| H | 0.971257 | 0.472534 | 0.222683 | 0.447693 | 2.621813 | 2.245 | 42.098 | 1104.938 | 0.000 | 0.0000 |
| C | 6.467461 | 3.353818 | 0.506661 | 0.000000 | 2.344966 | 23.494 | 353.376 | 4001.387 | 41152.121 | −1.2833 |
| Cl | 5.963451 | 3.862537 | 1.467911 | 1.098777 | 2.052787 | 93.240 | 1615.853 | 65715.929 | 1310829.439 | −1.2661 |
| **$CO_2$** | | | | | | | | | | |
| C | 2.944847 | 1.541728 | 1.090558 | 0.180486 | 2.329865 | 19.902 | 392.050 | 6560.549 | 144984.178 | −0.8645 |
| O | 4.810107 | 2.675187 | 0.377269 | 1.109199 | 2.489856 | 15.043 | 264.275 | 6361.827 | 104726.425 | −0.7611 |
| **Dimethyl Ether** | | | | | | | | | | |
| H | 0.581181 | 0.286373 | 0.143439 | 0.202139 | 2.167921 | 2.245 | 42.098 | 1104.938 | 0.000 | 0.0000 |
| C | 1.767333 | 1.211427 | 0.000000 | 0.000000 | 2.023109 | 23.494 | 353.376 | 4001.387 | 41152.121 | −1.3211 |
| O | 4.345253 | 2.836892 | 0.461020 | 1.090828 | 2.440026 | 12.235 | 266.573 | 6615.160 | 125669.048 | −0.0001 |
| **Ethane** | | | | | | | | | | |
| H | 0.631650 | 0.315461 | 0.131793 | 0.219936 | 2.230203 | 2.245 | 42.098 | 1104.938 | 0.000 | 0.0000 |
| C | 1.910136 | 1.281663 | 0.141830 | 0.053648 | 2.005074 | 23.494 | 353.376 | 4001.387 | 41152.121 | −1.2959 |
| **Ethanol** | | | | | | | | | | |
| CO | 2.913808 | 2.307707 | 0.000000 | 0.000000 | 2.238251 | 23.494 | 353.376 | 4001.387 | 41152.121 | −1.2545 |
| OH | 4.405898 | 2.864522 | 0.249909 | 0.990766 | 2.364797 | 14.592 | 320.063 | 8074.269 | 154258.592 | −0.8362 |
| HC | 0.567445 | 0.273172 | 0.150893 | 0.203159 | 2.206603 | 2.245 | 42.098 | 1104.938 | 0.000 | 0.0000 |
| HO | 0.202063 | 0.069581 | 0.160674 | 0.066068 | 2.044162 | 1.627 | 16.150 | 918.236 | 0.000 | 0.0000 |
| CH | 2.007588 | 1.232904 | 0.053800 | 0.111974 | 1.957305 | 23.494 | 353.376 | 4001.387 | 41152.121 | −1.1875 |
| **Ethene** | | | | | | | | | | |
| C | 2.776192 | 1.784015 | 0.373691 | 0.595405 | 1.917413 | 28.252 | 422.533 | 9835.457 | 152927.660 | −1.2627 |
| H | 0.631922 | 0.201132 | 0.133224 | 0.230793 | 2.464030 | 2.245 | 42.098 | 1104.938 | 0.000 | 0.0000 |
| **$H_2O$** | | | | | | | | | | |
| H | 0.272492 | 0.104357 | 0.179978 | 0.076004 | 2.167067 | 0.776 | 3.042 | 270.370 | 0.000 | 0.0000 |
| O | 3.837717 | 2.565879 | 0.049844 | 0.819591 | 2.288712 | 25.358 | 536.662 | 12267.338 | 220953.821 | −0.9794 |
| **Methane** | | | | | | | | | | |
| C | 2.117483 | 1.363604 | 0.080199 | 0.139272 | 1.916253 | 23.494 | 353.376 | 4001.387 | 41152.121 | −1.2959 |
| H | 0.832442 | 0.378112 | 0.197234 | 0.275122 | 2.444062 | 2.245 | 42.098 | 1104.938 | 0.000 | 0.0000 |
| **Methanol** | | | | | | | | | | |
| CO | 1.716271 | 1.018657 | 0.075645 | 0.000000 | 2.015251 | 23.494 | 353.376 | 4001.387 | 41152.121 | −1.2724 |
| OH | 4.379738 | 2.834034 | 0.232433 | 0.972620 | 2.373075 | 14.592 | 320.063 | 8074.269 | 154258.592 | −0.8102 |
| HO | 0.192535 | 0.064937 | 0.156032 | 0.067016 | 2.080537 | 1.627 | 16.150 | 918.236 | 0.000 | 0.0000 |
| HC | 0.572402 | 0.299836 | 0.151486 | 0.205148 | 2.201724 | 2.245 | 42.098 | 1104.938 | 0.000 | 0.0000 |

**Table S8 – continued from previous page**

| Atomtype | $A_{exch}$ | $A_{elst}$ | $A_{ind}$ | $A_{\delta HF}$ | $B$ | $C_6$ | $C_8$ | $C_{10}$ | $C_{12}$ | $Q_{drude}$ |
|---|---|---|---|---|---|---|---|---|---|---|
| **Methyl Amine** | | | | | | | | | | |
| HN | 0.297883 | 0.075404 | 0.157275 | 0.106014 | 2.264301 | 1.627 | 16.150 | 918.236 | 0.000 | 0.0000 |
| N | 3.141193 | 2.168747 | 0.193794 | 0.658763 | 2.020158 | 22.664 | 623.023 | 19359.417 | 472166.465 | −1.1026 |
| C | 2.331206 | 1.684778 | 0.103555 | 0.000000 | 2.048098 | 23.494 | 353.376 | 4001.387 | 41152.121 | −1.2667 |
| HC | 0.549424 | 0.253325 | 0.141786 | 0.212025 | 2.202002 | 2.245 | 42.098 | 1104.938 | 0.000 | 0.0000 |
| **$NH_3$** | | | | | | | | | | |
| H | 0.456908 | 0.162377 | 0.216086 | 0.153989 | 2.457227 | 1.627 | 16.150 | 918.236 | 0.000 | −1.1928 |
| N | 2.628746 | 1.857589 | 0.105469 | 0.514765 | 1.941661 | 22.664 | 623.023 | 19359.417 | 472166.465 | 0.0000 |

## S8.3 Born-Mayer-IP FF Parameters

$A_i$, $B_i$, $C_{i,n}$ parameters for the Born-Mayer-IP FF are listed in Table S9. $A_{ij}$, $B_{ij}$, and $C_{ij,n}$ parameters can be determined from the following combination rules:

$$A_{ij} = A_i A_j$$
$$B_{ij} = \frac{B_i B_j (B_i + B_j)}{B_i^2 + B_j^2}$$
$$C_{ij,n} = \sqrt{C_{i,n} C_{j,n}}$$

Parameters are given for each unique atom type in each molecule; where multiple atom types exist for a particular element, atom types are labeled first with the element name and second by connectivity. Thus the carbonyl carbon in acetone is labeled 'CO', whereas the methyl carbon is labeled 'CH'.

The total force field energy is defined by the following equations:

$$B_i = 2\sqrt{2IP_i}$$
$$P(B_{ij}, r_{ij}) = 1$$
$$x = B_{ij} r_{ij}$$
$$f_{2n}(x) = 1 - e^{-x} \sum_{k=0}^{2n} \frac{(x)^k}{k!}$$
$$V_{ij}^{\text{exch}} = A_{ij}^{exch} P(B_{ij}, r_{ij}) \exp(-B_{ij} r_{ij})$$
$$V_{ij}^{\text{elst}} = -A_{ij}^{elst} P(B_{ij}, r_{ij}) \exp(-B_{ij} r_{ij}) + \sum_{tu} Q_t^i T_{tu} Q_u^j$$
$$V_{ij}^{\text{ind}} = -A_{ij}^{ind} P(B_{ij}, r_{ij}) \exp(-B_{ij} r_{ij}) + V_{\text{shell}}^{(2)}$$
$$V_{ij}^{\delta\text{HF}} = -A_{ij}^{\delta\text{HF}} P(B_{ij}, r_{ij}) \exp(-B_{ij} r_{ij}) + V_{\text{shell}}^{(3-\infty)}$$
$$V_{ij}^{\text{disp}} = -\sum_{n=3}^{6} f_{2n}(x) \frac{C_{ij,2n}}{r_{ij}^{2n}}$$

$$V_{\text{FF}} = \sum_{ij} V_{ij}^{\text{elst}} + V_{ij}^{\text{exch}} + V_{ij}^{\text{ind}} + V_{ij}^{\delta\text{HF}} + V_{ij}^{\text{disp}}$$

The Tang-Toennies damping function $f$ is defined in the main text; the polarization energy $E_{pol}$ arising from drude oscillators is defined in ref. 1.

**Table S9.** Born-Mayer-IP FF parameters.

| Atomtype | $A_{exch}$ | $A_{elst}$ | $A_{ind}$ | $A_{\delta HF}$ | $B$ | $C_6$ | $C_8$ | $C_{10}$ | $C_{12}$ | $Q_{drude}$ |
|---|---|---|---|---|---|---|---|---|---|---|
| **Acetone** | | | | | | | | | | |
| CO | 5.567455 | 2.919090 | 2.729352 | 0.705232 | 1.819469 | 13.406 | 145.511 | 6091.546 | 80859.461 | −0.4541 |
| OC | 12.941114 | 8.025300 | 0.409461 | 3.556175 | 2.000912 | 22.881 | 353.876 | 10131.697 | 174478.272 | −0.9327 |
| CH | 10.952564 | 6.356726 | 0.000000 | 0.230007 | 1.819469 | 23.494 | 353.376 | 4001.387 | 41152.121 | −1.2947 |
| HC | 2.111731 | 1.047688 | 0.616407 | 0.767149 | 1.999464 | 2.245 | 42.098 | 1104.938 | 0.000 | 0.0000 |
| **Ar** | | | | | | | | | | |
| Ar | 50.711700 | 26.176317 | 5.968585 | 9.099102 | 2.152496 | 71.007 | 1556.382 | 37687.507 | 709695.360 | −1.0694 |
| **Chloromethane** | | | | | | | | | | |
| H | 1.773426 | 0.876699 | 0.418998 | 0.906852 | 1.999464 | 2.245 | 42.098 | 1104.938 | 0.000 | 0.0000 |
| C | 12.813654 | 7.191403 | 1.079346 | 0.000000 | 1.819469 | 23.494 | 353.376 | 4001.387 | 41152.121 | −1.2833 |
| Cl | 34.276817 | 20.817366 | 7.997654 | 5.798695 | 1.952538 | 93.240 | 1615.853 | 65715.929 | 1310829.439 | −1.2661 |
| **$CO_2$** | | | | | | | | | | |
| C | 5.176487 | 2.984618 | 2.277174 | 0.274561 | 1.819469 | 19.902 | 392.050 | 6560.549 | 144984.178 | −0.8645 |
| O | 11.349651 | 6.499242 | 0.865006 | 2.716049 | 2.000912 | 15.043 | 264.275 | 6361.827 | 104726.425 | −0.7611 |
| **Dimethyl Ether** | | | | | | | | | | |
| H | 2.329781 | 1.183750 | 0.564499 | 0.806639 | 1.999464 | 2.245 | 42.098 | 1104.938 | 0.000 | 0.0000 |
| C | 8.563364 | 4.968189 | 0.131071 | 0.074779 | 1.819469 | 23.494 | 353.376 | 4001.387 | 41152.121 | −1.3211 |
| O | 11.989376 | 7.808839 | 1.317489 | 3.114127 | 2.000912 | 12.235 | 266.573 | 6615.160 | 125669.048 | −0.0001 |
| **Ethane** | | | | | | | | | | |
| H | 2.250973 | 1.158733 | 0.485471 | 0.781917 | 1.999464 | 2.245 | 42.098 | 1104.938 | 0.000 | 0.0000 |
| C | 10.461511 | 5.586592 | 0.612844 | 0.406278 | 1.819469 | 23.494 | 353.376 | 4001.387 | 41152.121 | −1.2959 |
| **Ethanol** | | | | | | | | | | |
| CO | 8.222663 | 5.833862 | 0.000000 | 0.000000 | 1.819469 | 23.494 | 353.376 | 4001.387 | 41152.121 | −1.2545 |
| OH | 13.923864 | 8.979075 | 0.940969 | 3.229934 | 2.000912 | 14.592 | 320.063 | 8074.269 | 154258.592 | −0.8362 |
| HC | 2.149784 | 1.068436 | 0.570784 | 0.766874 | 1.999464 | 2.245 | 42.098 | 1104.938 | 0.000 | 0.0000 |
| HO | 1.019177 | 0.356079 | 0.751733 | 0.328847 | 1.999464 | 1.627 | 16.150 | 918.236 | 0.000 | 0.0000 |
| CH | 10.141256 | 5.806452 | 0.278019 | 0.593277 | 1.819469 | 23.494 | 353.376 | 4001.387 | 41152.121 | −1.1875 |
| **Ethene** | | | | | | | | | | |
| C | 15.765638 | 9.111034 | 1.960627 | 2.997793 | 1.819469 | 28.252 | 422.533 | 9835.457 | 152927.660 | −1.2627 |
| H | 1.601044 | 0.584328 | 0.335499 | 0.611640 | 1.999464 | 2.245 | 42.098 | 1104.938 | 0.000 | 0.0000 |
| **$H_2O$** | | | | | | | | | | |
| H | 1.141499 | 0.446043 | 0.697274 | 0.318684 | 1.999464 | 0.776 | 3.042 | 270.370 | 0.000 | 0.0000 |
| O | 13.932606 | 9.201940 | 0.282581 | 2.951132 | 2.000912 | 25.358 | 536.662 | 12267.338 | 220953.821 | −0.9794 |
| **Methane** | | | | | | | | | | |
| C | 11.713473 | 6.761088 | 0.527832 | 0.632892 | 1.819469 | 23.494 | 353.376 | 4001.387 | 41152.121 | −1.2959 |
| H | 2.225001 | 1.035042 | 0.508080 | 0.739327 | 1.999464 | 2.245 | 42.098 | 1104.938 | 0.000 | 0.0000 |
| **Methanol** | | | | | | | | | | |
| CO | 7.433631 | 4.180536 | 0.401704 | 0.000000 | 1.819469 | 23.494 | 353.376 | 4001.387 | 41152.121 | −1.2724 |
| OH | 13.542794 | 8.726014 | 0.795157 | 3.058222 | 2.000912 | 14.592 | 320.063 | 8074.269 | 154258.592 | −0.8102 |
| HO | 0.922058 | 0.309528 | 0.702616 | 0.306417 | 1.999464 | 1.627 | 16.150 | 918.236 | 0.000 | 0.0000 |
| HC | 2.230349 | 1.176985 | 0.567045 | 0.789220 | 1.999464 | 2.245 | 42.098 | 1104.938 | 0.000 | 0.0000 |
| **Methyl Amine** | | | | | | | | | | |

**Table S9 – continued from previous page**

| Atomtype | $A_{exch}$ | $A_{elst}$ | $A_{ind}$ | $A_{\delta HF}$ | $B$ | $C_6$ | $C_8$ | $C_{10}$ | $C_{12}$ | $Q_{drude}$ |
|---|---|---|---|---|---|---|---|---|---|---|
| HN | 1.224682 | 0.421352 | 0.547503 | 0.429622 | 1.999464 | 1.627 | 16.150 | 918.236 | 0.000 | 0.0000 |
| N | 23.338368 | 15.290981 | 1.429713 | 4.422039 | 2.067111 | 22.664 | 623.023 | 19359.417 | 472166.465 | −1.1026 |
| C | 10.818390 | 6.130391 | 0.375108 | 0.000000 | 1.819469 | 23.494 | 353.376 | 4001.387 | 41152.121 | −1.2667 |
| HC | 2.000843 | 1.025883 | 0.546828 | 0.808373 | 1.999464 | 2.245 | 42.098 | 1104.938 | 0.000 | 0.0000 |
| **$NH_3$** | | | | | | | | | | |
| H | 1.291205 | 0.567250 | 0.560466 | 0.444433 | 1.999464 | 1.627 | 16.150 | 918.236 | 0.000 | −1.1928 |
| N | 23.837579 | 14.999330 | 0.902266 | 4.021003 | 2.067111 | 22.664 | 623.023 | 19359.417 | 472166.465 | 0.0000 |

## S8.4 Born-Mayer-sISA FF Parameters

$A_i$, $B_i$, $C_{i,n}$ parameters for the Born-Mayer-sISA FF are listed in Table S10. $A_{ij}$, $B_{ij}$, and $C_{ij,n}$ parameters can be determined from the following combination rules:

$$\begin{aligned} A_{ij} &= A_i A_j \\ B_{ij} &= \sqrt{B_i B_j} \\ C_{ij,n} &= \sqrt{C_{i,n} C_{j,n}} \end{aligned}$$

Parameters are given for each unique atom type in each molecule; where multiple atom types exist for a particular element, atom types are labeled first with the element name and second by connectivity. Thus the carbonyl carbon in acetone is labeled 'CO', whereas the methyl carbon is labeled 'CH'.

The total force field energy is defined by the following equations:

$$\begin{aligned} B_i &= 0.84 B_i^{ISA} \\ P(B_{ij}, r_{ij}) &= 1 \\ x &= B_{ij} r_{ij} \\ f_{2n}(x) &= 1 - e^{-x} \sum_{k=0}^{2n} \frac{(x)^k}{k!} \\ V_{ij}^{\text{exch}} &= A_{ij}^{exch} P(B_{ij}, r_{ij}) \exp(-B_{ij} r_{ij}) \\ V_{ij}^{\text{elst}} &= -A_{ij}^{elst} P(B_{ij}, r_{ij}) \exp(-B_{ij} r_{ij}) + \sum_{tu} Q_t^i T_{tu} Q_u^j \\ V_{ij}^{\text{ind}} &= -A_{ij}^{ind} P(B_{ij}, r_{ij}) \exp(-B_{ij} r_{ij}) + V_{\text{shell}}^{(2)} \\ V_{ij}^{\delta\text{HF}} &= -A_{ij}^{\delta\text{HF}} P(B_{ij}, r_{ij}) \exp(-B_{ij} r_{ij}) + V_{\text{shell}}^{(3-\infty)} \\ V_{ij}^{\text{disp}} &= -\sum_{n=3}^{6} f_{2n}(x) \frac{C_{ij,2n}}{r_{ij}^{2n}} \end{aligned}$$

$$V_{\text{FF}} = \sum_{ij} V_{ij}^{\text{elst}} + V_{ij}^{\text{exch}} + V_{ij}^{\text{ind}} + V_{ij}^{\delta\text{HF}} + V_{ij}^{\text{disp}}$$

The Tang-Toennies damping function $f$ is defined in the main text; the polarization energy $V_{\text{shell}} = V_{\text{shell}}^{(2)} + V_{\text{shell}}^{(3-\infty)}$ arising from drude oscillators is defined in ref. 1.

**Table S10.** Born-Mayer-sISA FF parameters.

| Atomtype | $A_{exch}$ | $A_{elst}$ | $A_{ind}$ | $A_{\delta HF}$ | $B$ | $C_6$ | $C_8$ | $C_{10}$ | $C_{12}$ | $Q_{drude}$ |
|---|---|---|---|---|---|---|---|---|---|---|
| **Acetone** | | | | | | | | | | |
| CO | 11.298138 | 6.260674 | 6.375244 | 1.474927 | 2.187934 | 13.406 | 145.511 | 6091.546 | 80859.461 | −0.4541 |
| OC | 12.485402 | 7.747160 | 0.426691 | 3.414128 | 1.982936 | 22.881 | 353.876 | 10131.697 | 174478.272 | −0.9327 |
| CH | 6.752770 | 3.978541 | 0.000000 | 0.139991 | 1.623387 | 23.494 | 353.376 | 4001.387 | 41152.121 | −1.2947 |
| HC | 1.703654 | 0.836792 | 0.517761 | 0.641695 | 1.904091 | 2.245 | 42.098 | 1104.938 | 0.000 | 0.0000 |
| **Ar** | | | | | | | | | | |
| Ar | 17.754951 | 10.759634 | 2.431058 | 3.745351 | 1.833974 | 71.007 | 1556.382 | 37687.507 | 709695.360 | −1.0694 |
| **Chloromethane** | | | | | | | | | | |
| H | 2.839538 | 1.357582 | 0.664424 | 1.323373 | 2.202323 | 2.245 | 42.098 | 1104.938 | 0.000 | 0.0000 |
| C | 19.308314 | 10.282602 | 1.457576 | 0.000000 | 1.969771 | 23.494 | 353.376 | 4001.387 | 41152.121 | −1.2833 |
| Cl | 17.706793 | 11.554461 | 4.398795 | 3.296506 | 1.724341 | 93.240 | 1615.853 | 65715.929 | 1310829.439 | −1.2661 |
| **$CO_2$** | | | | | | | | | | |
| C | 8.367127 | 4.534796 | 3.258447 | 0.502437 | 1.957087 | 19.902 | 392.050 | 6560.549 | 144984.178 | −0.8645 |
| O | 14.291097 | 8.007681 | 1.115752 | 3.326093 | 2.091479 | 15.043 | 264.275 | 6361.827 | 104726.425 | −0.7611 |
| **Dimethyl Ether** | | | | | | | | | | |
| H | 1.669015 | 0.824934 | 0.413473 | 0.583661 | 1.821054 | 2.245 | 42.098 | 1104.938 | 0.000 | 0.0000 |
| C | 5.566661 | 3.695046 | 0.009130 | 0.000000 | 1.699411 | 23.494 | 353.376 | 4001.387 | 41152.121 | −1.3211 |
| O | 12.945665 | 8.498393 | 1.411434 | 3.323600 | 2.049622 | 12.235 | 266.573 | 6615.160 | 125669.048 | −0.0001 |
| **Ethane** | | | | | | | | | | |
| H | 1.817180 | 0.907864 | 0.387236 | 0.628205 | 1.873370 | 2.245 | 42.098 | 1104.938 | 0.000 | 0.0000 |
| C | 6.043273 | 3.920646 | 0.401363 | 0.227334 | 1.684262 | 23.494 | 353.376 | 4001.387 | 41152.121 | −1.2959 |
| **Ethanol** | | | | | | | | | | |
| CO | 9.226602 | 7.053649 | 0.000000 | 0.000000 | 1.880131 | 23.494 | 353.376 | 4001.387 | 41152.121 | −1.2545 |
| OH | 13.217432 | 8.587995 | 0.791412 | 3.010794 | 1.986430 | 14.592 | 320.063 | 8074.269 | 154258.592 | −0.8362 |
| HC | 1.619514 | 0.783441 | 0.436133 | 0.585641 | 1.853547 | 2.245 | 42.098 | 1104.938 | 0.000 | 0.0000 |
| HO | 0.577312 | 0.197433 | 0.455572 | 0.189697 | 1.717096 | 1.627 | 16.150 | 918.236 | 0.000 | 0.0000 |
| CH | 6.248381 | 3.766536 | 0.169208 | 0.364715 | 1.644136 | 23.494 | 353.376 | 4001.387 | 41152.121 | −1.1875 |
| **Ethene** | | | | | | | | | | |
| C | 8.247499 | 5.331602 | 1.119056 | 1.784735 | 1.610627 | 28.252 | 422.533 | 9835.457 | 152927.660 | −1.2627 |
| H | 1.870937 | 0.594220 | 0.392884 | 0.678627 | 2.069785 | 2.245 | 42.098 | 1104.938 | 0.000 | 0.0000 |
| **$H_2O$** | | | | | | | | | | |
| H | 0.788146 | 0.300709 | 0.513573 | 0.220782 | 1.820336 | 0.776 | 3.042 | 270.370 | 0.000 | 0.0000 |
| O | 11.526687 | 7.698249 | 0.177170 | 2.460372 | 1.922518 | 25.358 | 536.662 | 12267.338 | 220953.821 | −0.9794 |
| **Methane** | | | | | | | | | | |
| C | 6.266192 | 4.123257 | 0.269389 | 0.480514 | 1.609652 | 23.494 | 353.376 | 4001.387 | 41152.121 | −1.2959 |
| H | 2.471370 | 1.103960 | 0.572840 | 0.792712 | 2.053012 | 2.245 | 42.098 | 1104.938 | 0.000 | 0.0000 |
| **Methanol** | | | | | | | | | | |
| CO | 5.275558 | 3.097679 | 0.245621 | 0.000000 | 1.692810 | 23.494 | 353.376 | 4001.387 | 41152.121 | −1.2724 |
| OH | 13.144521 | 8.507288 | 0.717814 | 2.940249 | 1.993383 | 14.592 | 320.063 | 8074.269 | 154258.592 | −0.8102 |
| HO | 0.548765 | 0.182757 | 0.445382 | 0.190565 | 1.747651 | 1.627 | 16.150 | 918.236 | 0.000 | 0.0000 |
| HC | 1.656132 | 0.867569 | 0.436199 | 0.594834 | 1.849448 | 2.245 | 42.098 | 1104.938 | 0.000 | 0.0000 |
| **Methyl Amine** | | | | | | | | | | |

Table S10 – continued from previous page

| Atomtype | $A_{exch}$ | $A_{elst}$ | $A_{ind}$ | $A_{\delta HF}$ | $B$ | $C_6$ | $C_8$ | $C_{10}$ | $C_{12}$ | $Q_{drude}$ |
|---|---|---|---|---|---|---|---|---|---|---|
| HN | 0.868281 | 0.222074 | 0.455689 | 0.311158 | 1.902013 | 1.627 | 16.150 | 918.236 | 0.000 | 0.0000 |
| N | 9.399190 | 6.470677 | 0.592158 | 1.969396 | 1.696933 | 22.664 | 623.023 | 19359.417 | 472166.465 | −1.1026 |
| C | 7.274600 | 5.119244 | 0.292498 | 0.000000 | 1.720403 | 23.494 | 353.376 | 4001.387 | 41152.121 | −1.2667 |
| HC | 1.572214 | 0.728368 | 0.413461 | 0.613379 | 1.849682 | 2.245 | 42.098 | 1104.938 | 0.000 | 0.0000 |
| **$NH_3$** | | | | | | | | | | |
| H | 1.346119 | 0.487459 | 0.631866 | 0.455708 | 2.064071 | 1.627 | 16.150 | 918.236 | 0.000 | −1.1928 |
| N | 7.875825 | 5.515104 | 0.323871 | 1.528953 | 1.630995 | 22.664 | 623.023 | 19359.417 | 472166.465 | 0.0000 |

# S9 Force Field Fits for Homomonomeric Systems

Scatter plots are shown for each homomonomeric system as an indication of force field quality with respect to DFT-SAPT (PBE0/AC) benchmark energies (Figure S4). As in the main text, fits for each energy component are displayed along with two views of the total interaction energy.

**(a)** Acetone Dimer

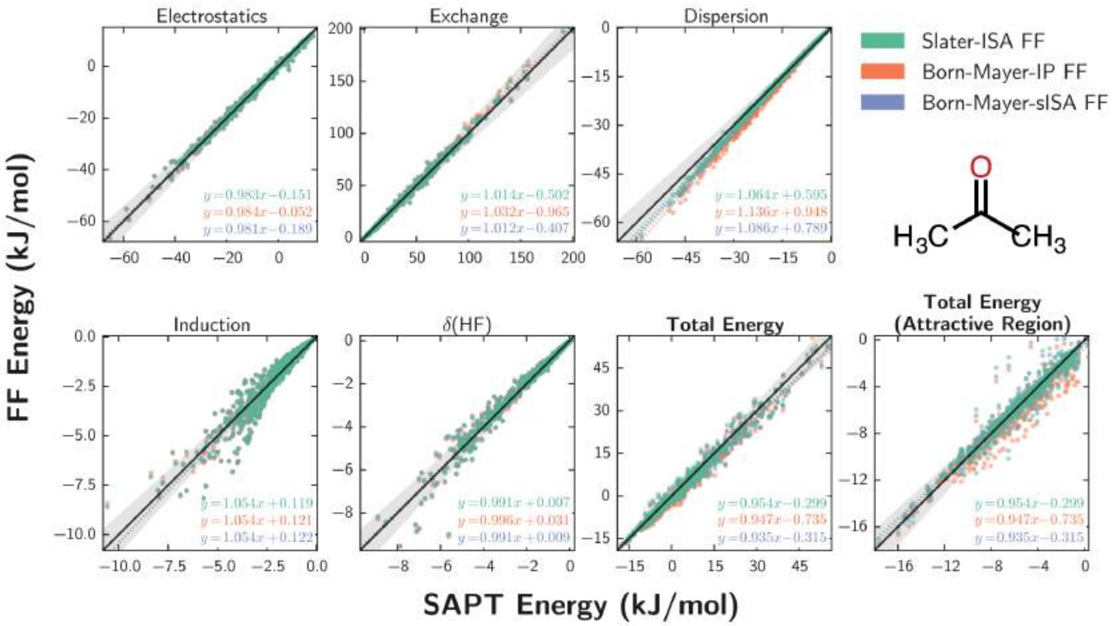


**(b)** Ar Dimer

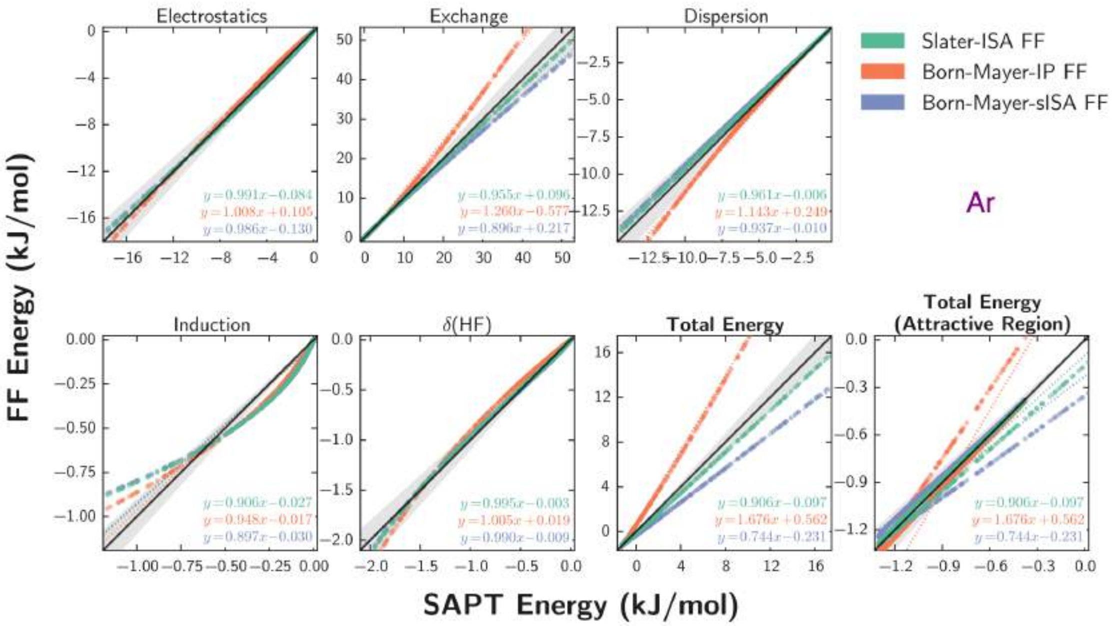

**(c)** Chloromethane Dimer

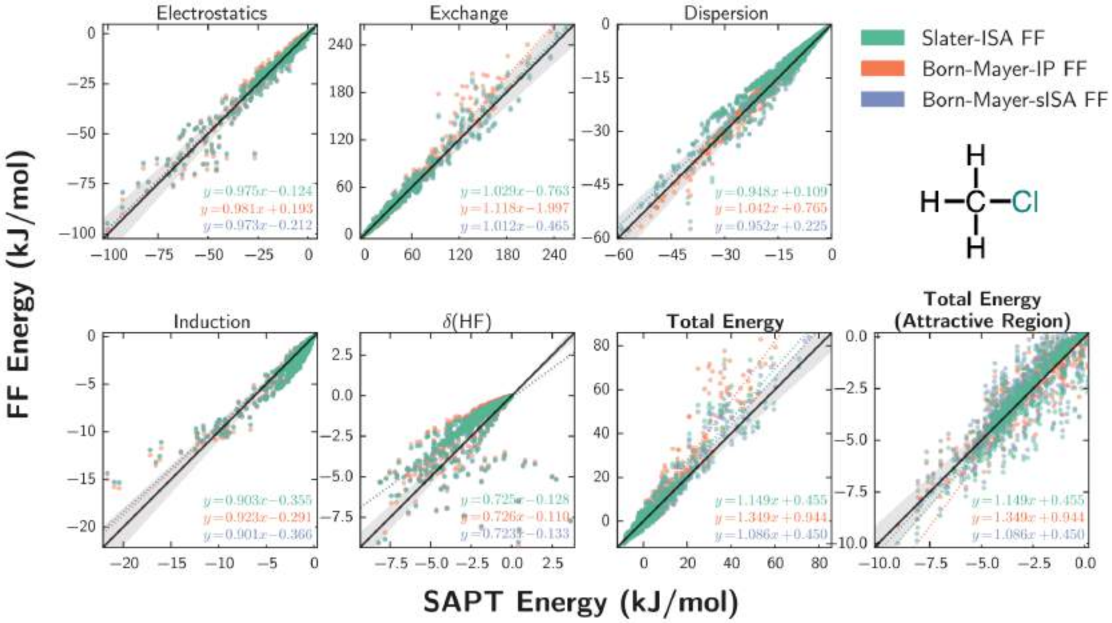


**(d)** $CO_2$ Dimer

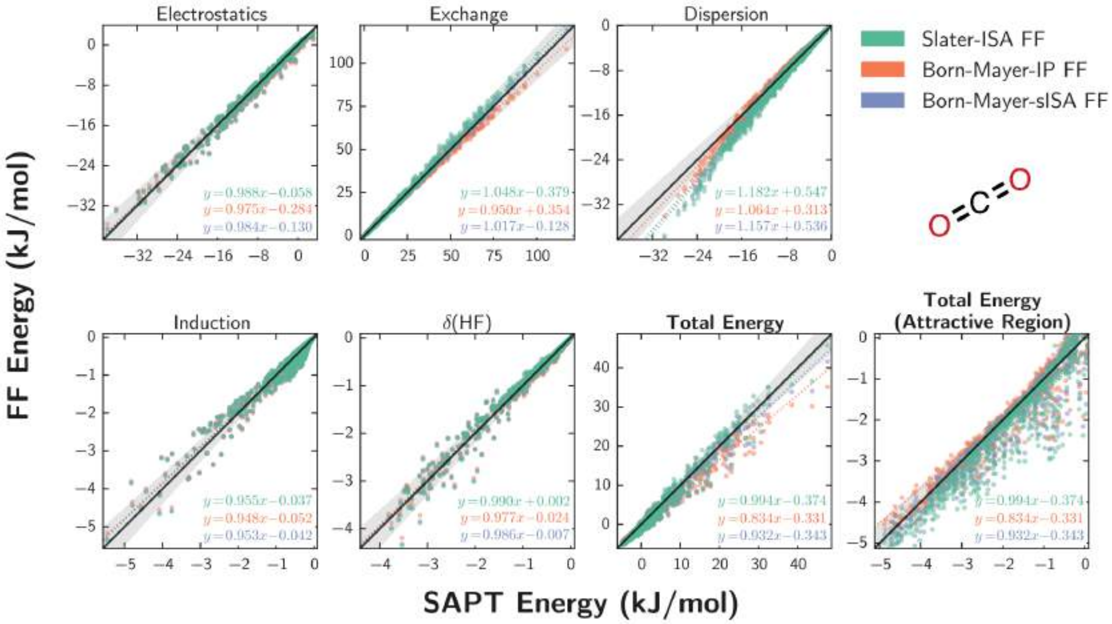

**(e)** Dimethyl Ether Dimer

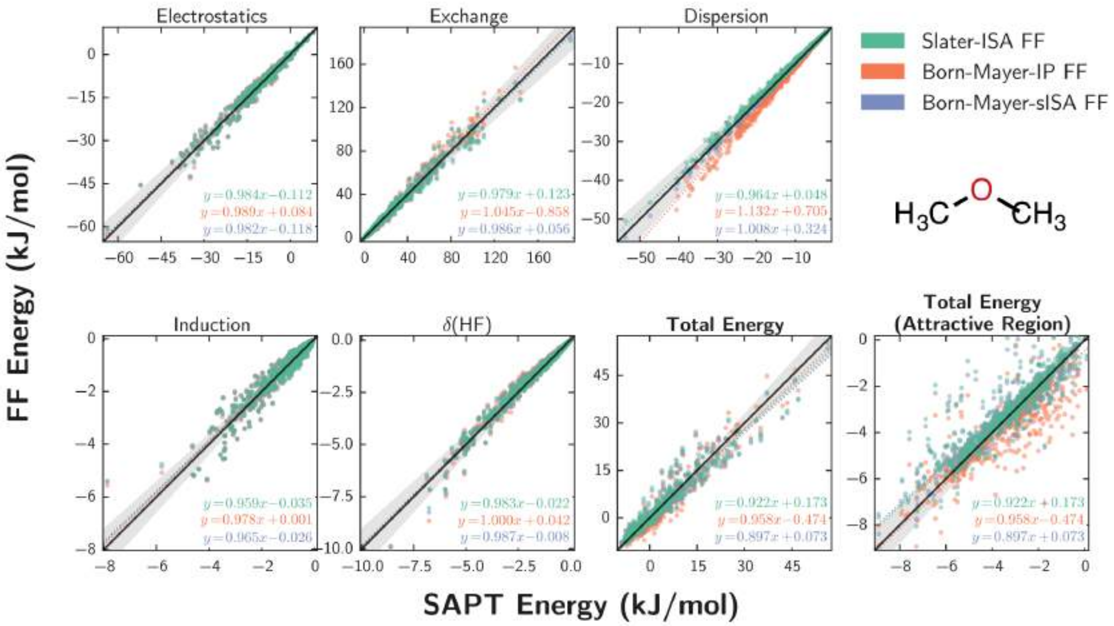


**(f)** Ethane Dimer

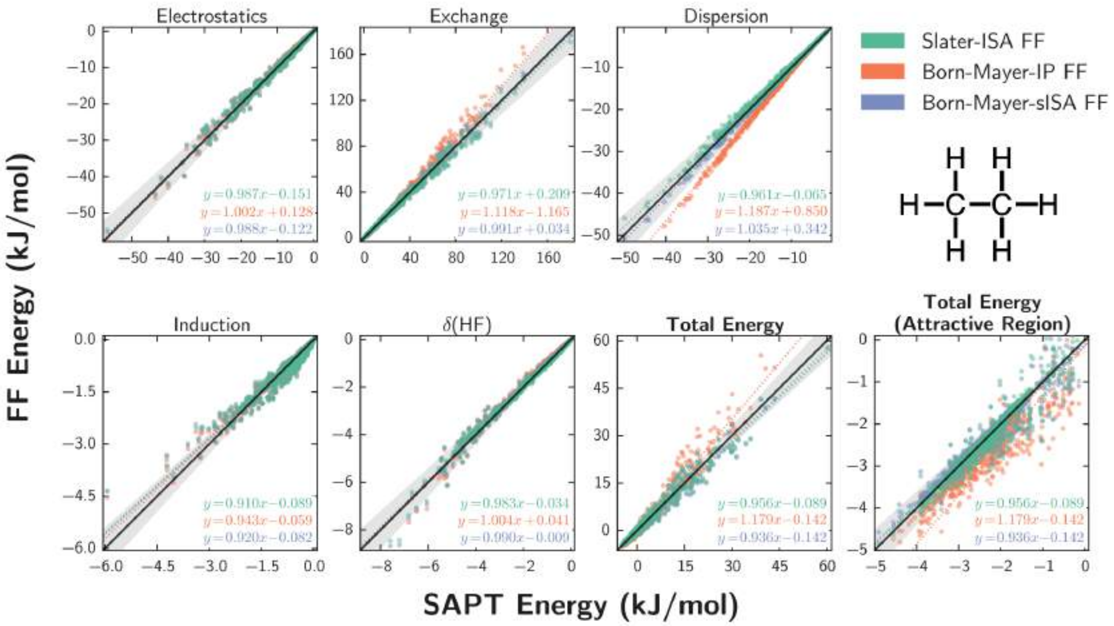

**(g)** Ethanol Dimer

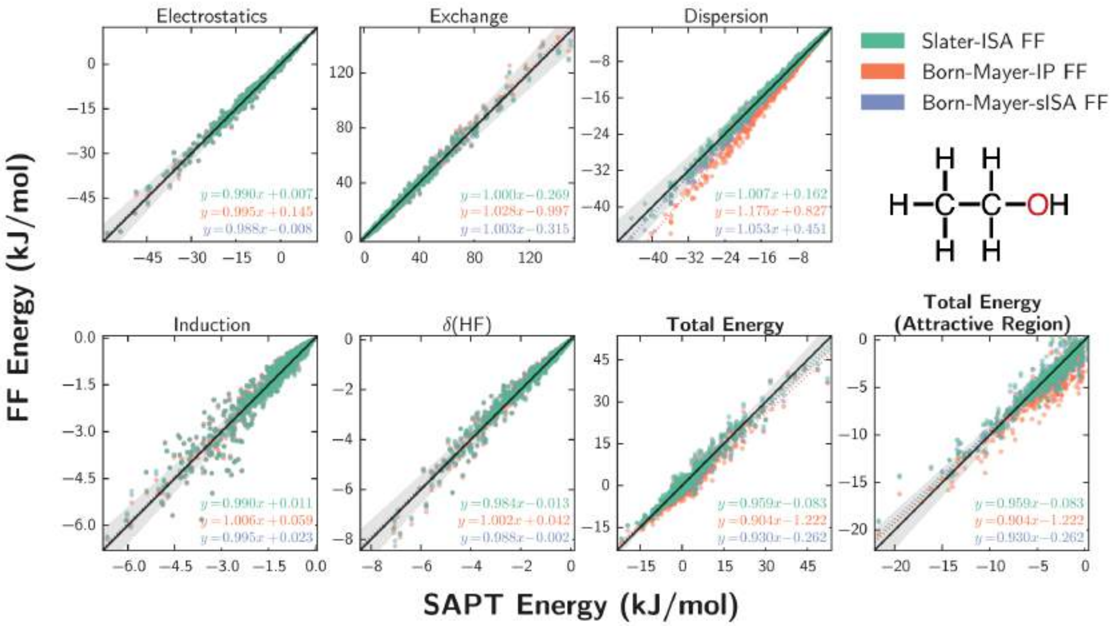


**(h)** Ethene Dimer

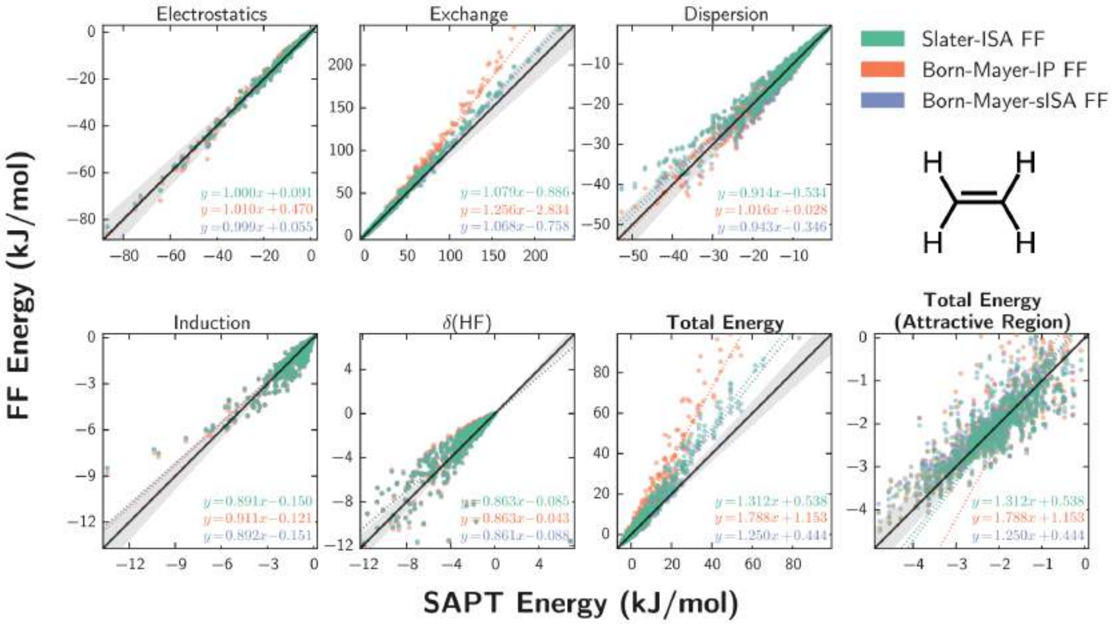

**(i)** $H_2O$ Dimer

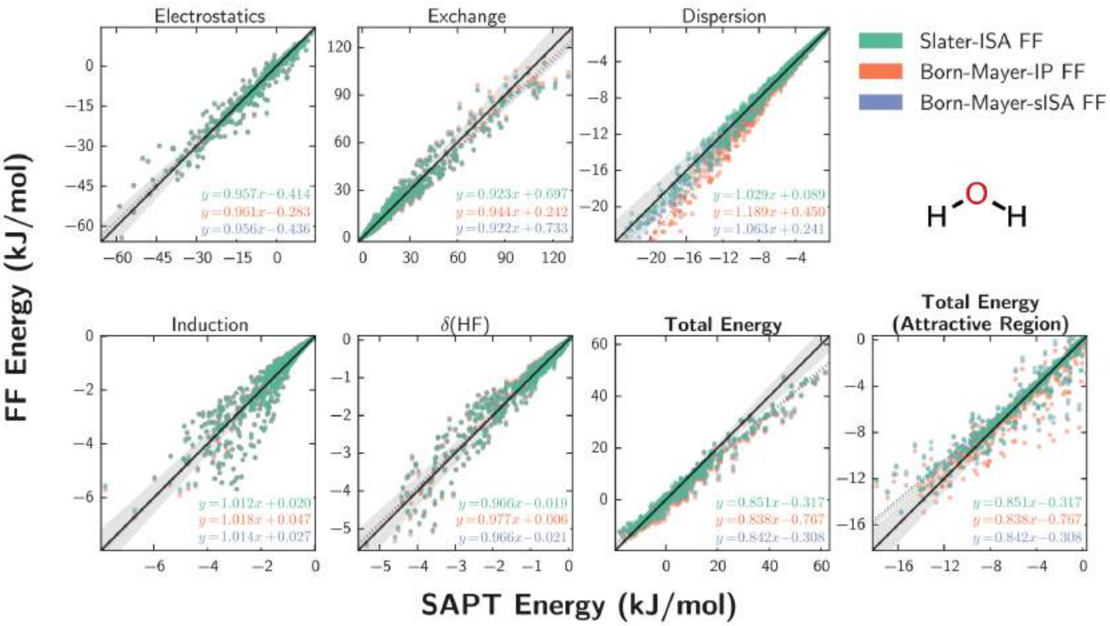


**(j)** Methane Dimer

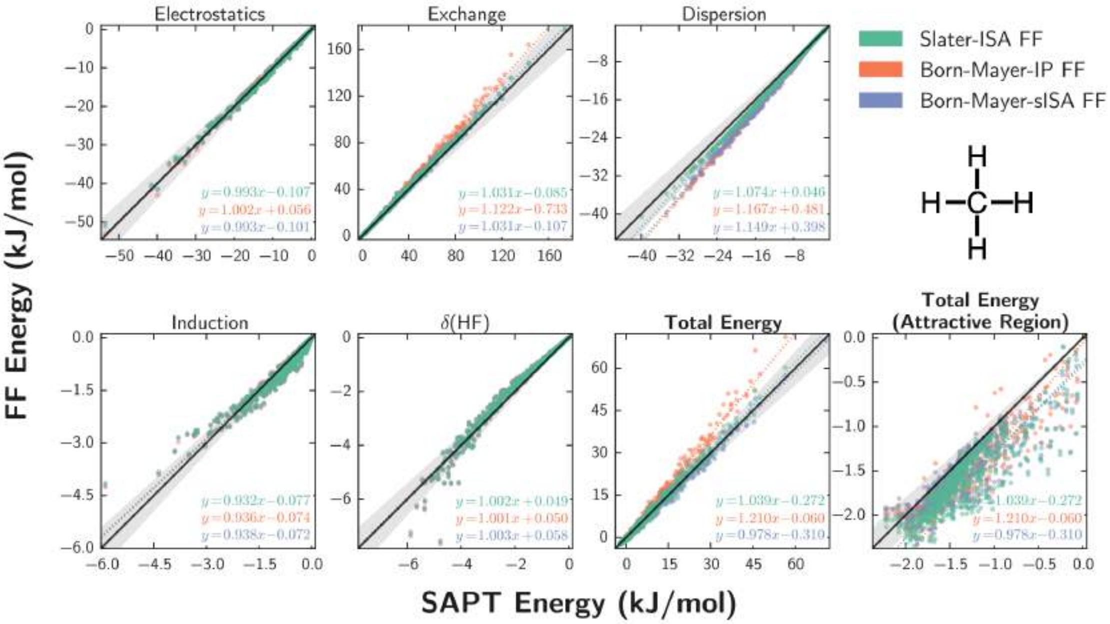

**(k)** Methanol Dimer

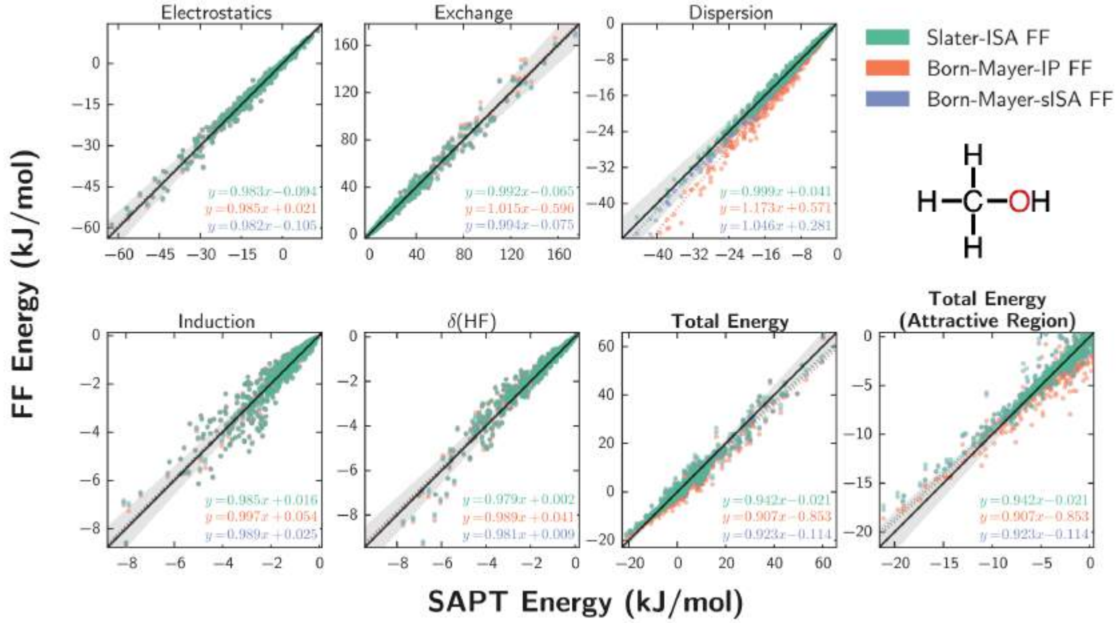


**(l)** Methyl Amine Dimer

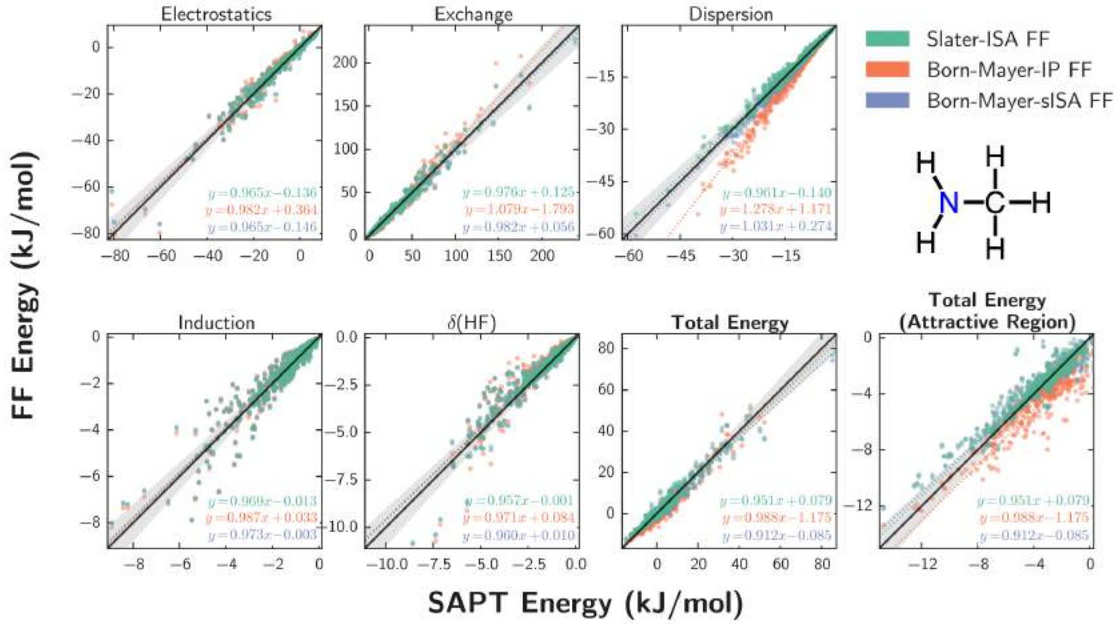

**(m)** $NH_3$ Dimer

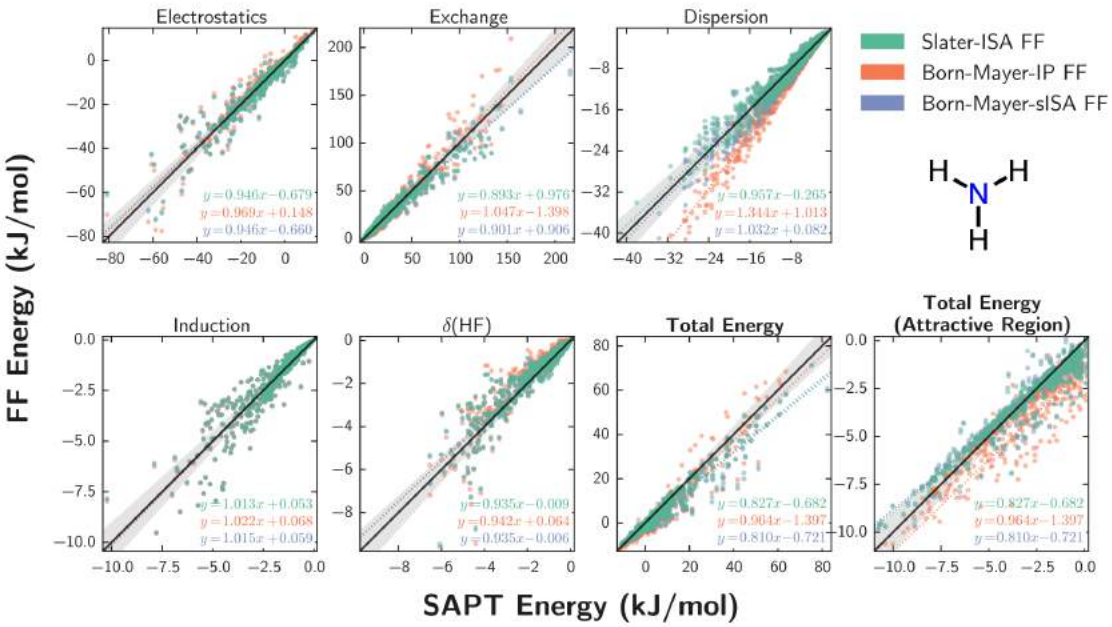


**Figure S4.** Force field fits for the homomoneric systems using the Slater-ISA FF (green), Born-Mayer-IP FF (orange) and Born-Mayer-sISA FF (blue). Fits for each energy component are displayed along with two views of the total interaction energy. The $y = x$ line (black) indicates perfect agreement between reference energies and each force field, while shaded grey areas represent points within ±10% agreement of the benchmark. To guide the eye, a line of best fit (dotted line) has been computed for each force field and for each energy component.

# S10 Force Field Accuracy for LJ FF

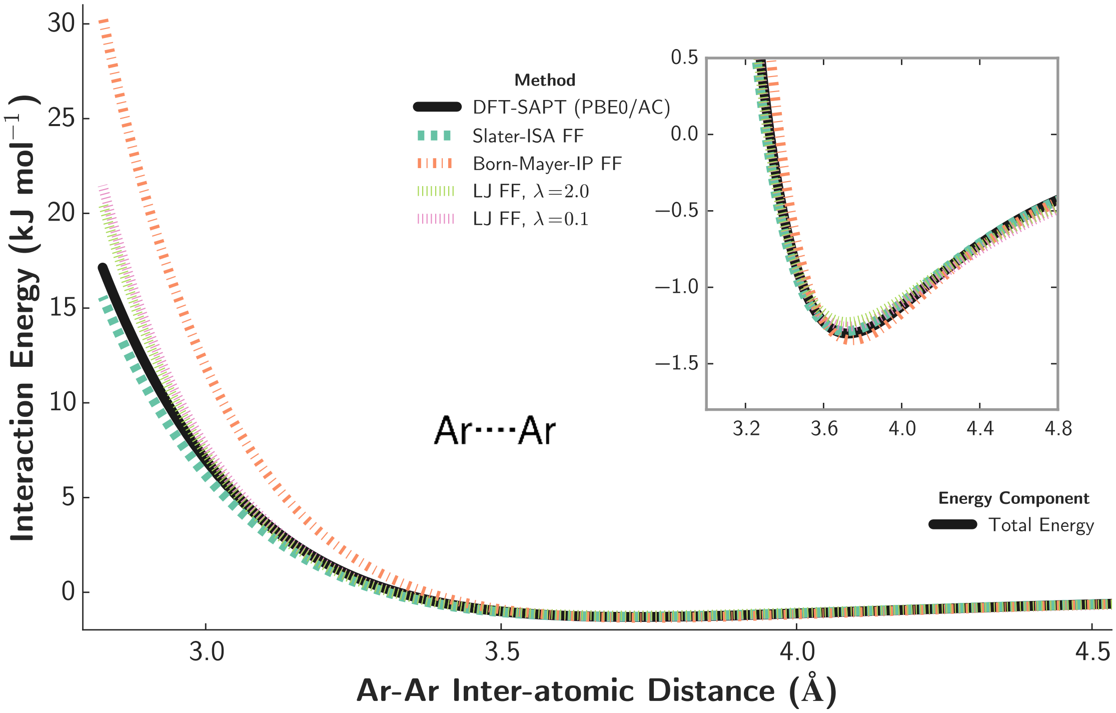


**Figure S5.** Potential energy surface for the argon dimer. Interaction energies for the Slater-ISA FF (dashed curves), Born-Mayer-IP FF (dash-dotted curves), and LJ FF (dotted curves) are shown alongside benchmark DFT-SAPT (PBE0/AC) energies (solid curves). Note that, for the LJ FF force fields, the magnitude of the attractive tail region is overestimated by the effective $C_{ij,6}$ dispersion parameter.

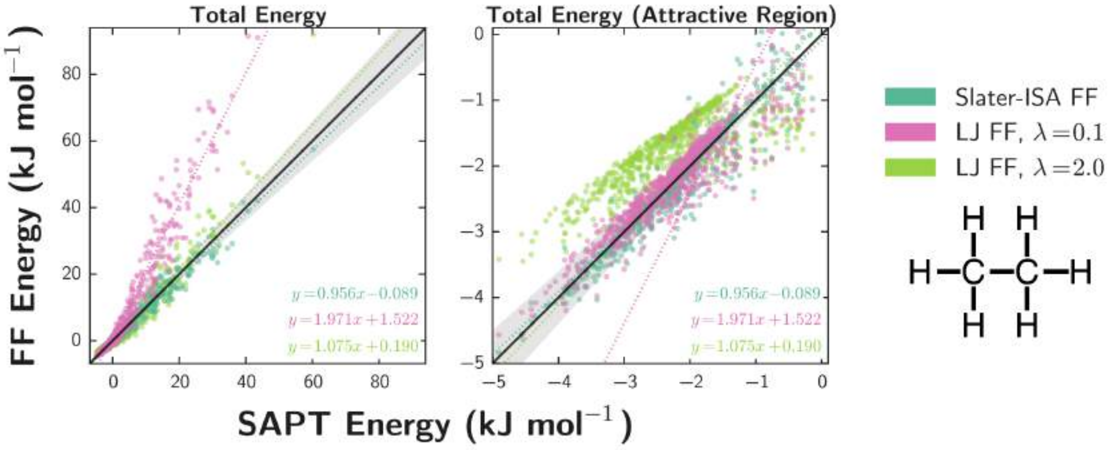


**Figure S6.** Fits for two views of the total interaction energy for the ethane dimer using the Slater-ISA (teal), LJ $\lambda = 0.1$ (pink) and LJ $\lambda = 2.0$ (lime green) FFs. The diagonal line (black) indicates perfect agreement between reference energies and each force field, while shaded grey areas represent points within ±10% agreement of the benchmark. To guide the eye, a line of best fit (dotted line) has been computed for each force field.

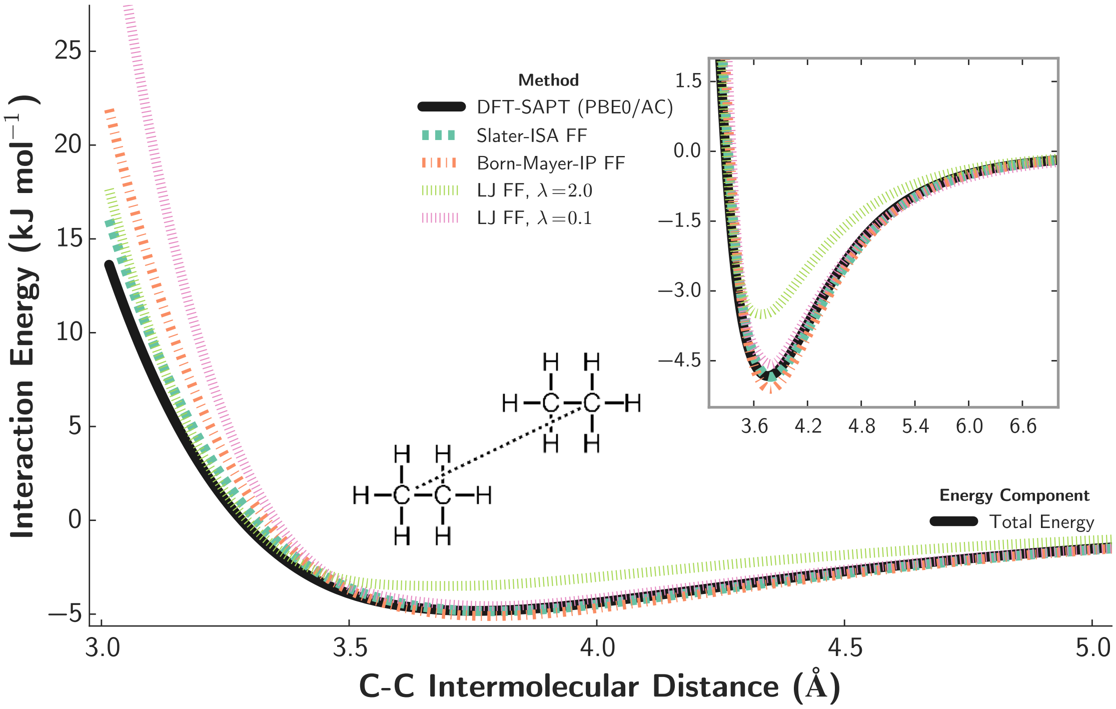


**Figure S7.** A representative potential energy scan near a local minimum for the ethane dimer. Interaction energies for the Slater-ISA FF (dashed curves), Born-Mayer-IP FF (dash-dotted curves), and LJ FF (dotted curves) are shown alongside benchmark DFT-SAPT (PBE0/AC) energies (solid curves). The energy decomposition for DFT-SAPT and for each force field is shown for reference. The ethane dimer configuration in this scan corresponds to the most energetically attractive dimer included in the training set; other points along this scan are not included in the training set.

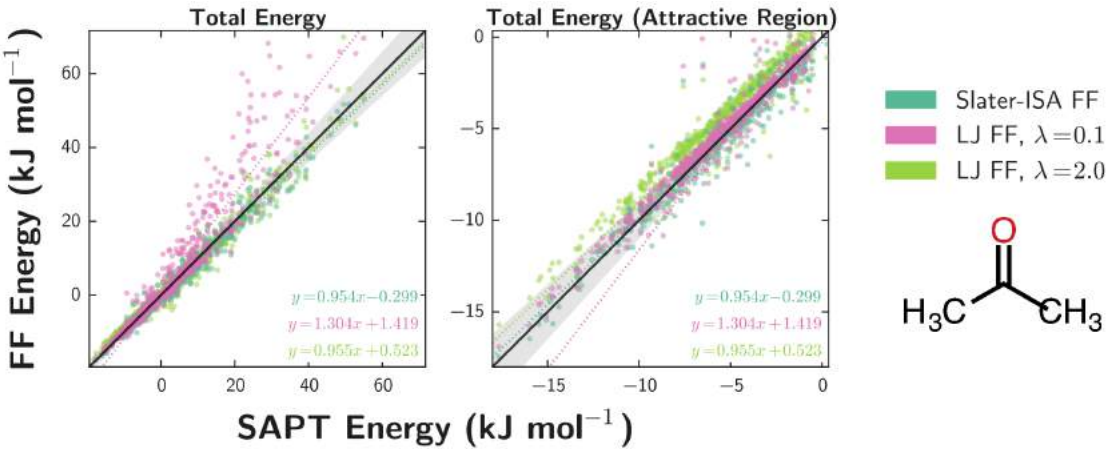


**Figure S8.** Force field fits for the acetone dimer using the Slater-ISA (teal), LJ $\lambda = 0.1$ (pink) and LJ $\lambda = 2.0$ (lime green) FFs. Fits for two views of the total interaction energy are displayed. The diagonal line (black) indicates perfect agreement between reference energies and each force field, while shaded grey areas represent points within $\pm 10\%$ agreement of the benchmark. To guide the eye, a line of best fit (dotted line) has been computed for each force field.

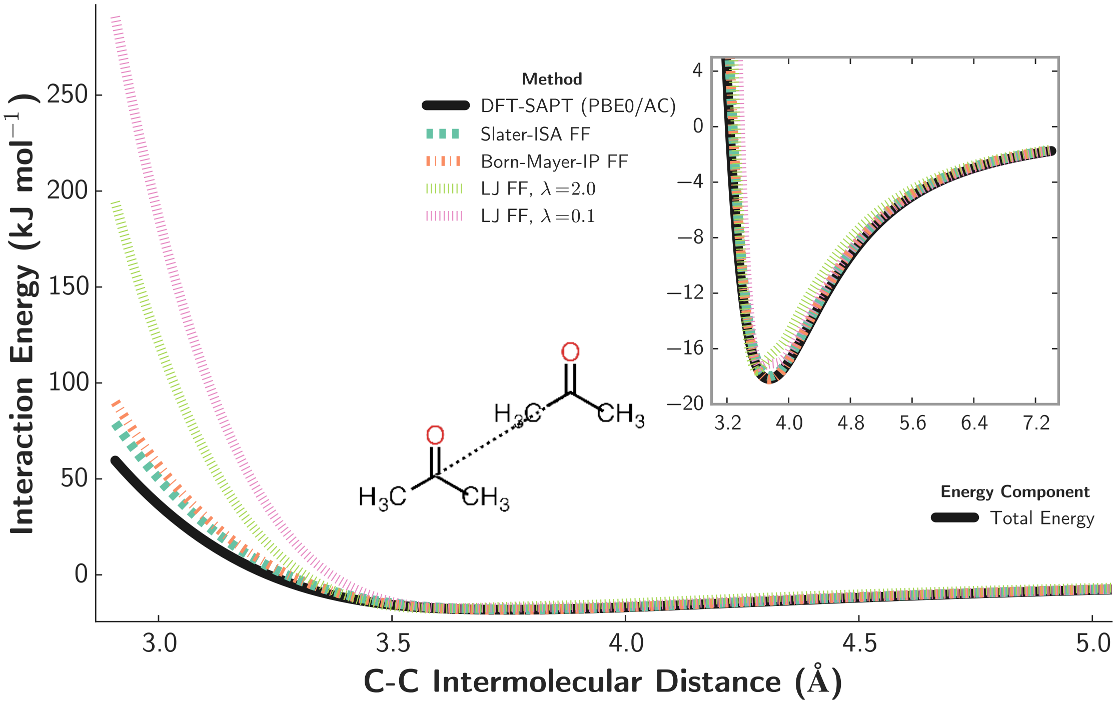


**Figure S9.** A representative potential energy scan near a local minimum for the acetone dimer. Interaction energies for the Slater-ISA FF (dashed curves), Born-Mayer-IP FF (dash-dotted curves), and LJ FF (dotted curves) are shown alongside benchmark DFT-SAPT (PBE0/AC) energies (solid curves). The energy decomposition for DFT-SAPT and for each force field is shown for reference. The intermolecular distance is taken to be the internuclear distance between the two carbonyl carbons on each acetone monomer. The acetone dimer configuration in this scan corresponds to the most energetically attractive dimer included in the training set; other points along this scan are not included in the training set.

## S11 Parameter Robustness for Argon

Argon parameters were tested for robustness by changing the weighting function as described in the main text. As with ethane, optimized Slater-ISA FF $A_{ij}$ parameters are much less sensitive to the choice of weighting function compared to the Born-Mayer-IP FF. As a result, the Slater-ISA FF shows decreased uncertainty when computing the 2$^{\text{nd}}$ virial coefficient. Virial coefficients for the Born-Mayer-IP FF, on the other hand, depend more strongly on the choice of weighting function. The fortuitous agreement with experiment for the Born-Mayer-IP FF with $\lambda = 0.5$ may point to inaccuracies in the DFT-SAPT potential itself, but is not indicative of enhanced force field fitting quality. (Indeed, Figure S11 shows that this weighting function leads to the worst agreement with DFT-SAPT compared to other $\lambda$ values). Overall, the argon fits demonstrate increased parameter robustness for the Slater-ISA FF.

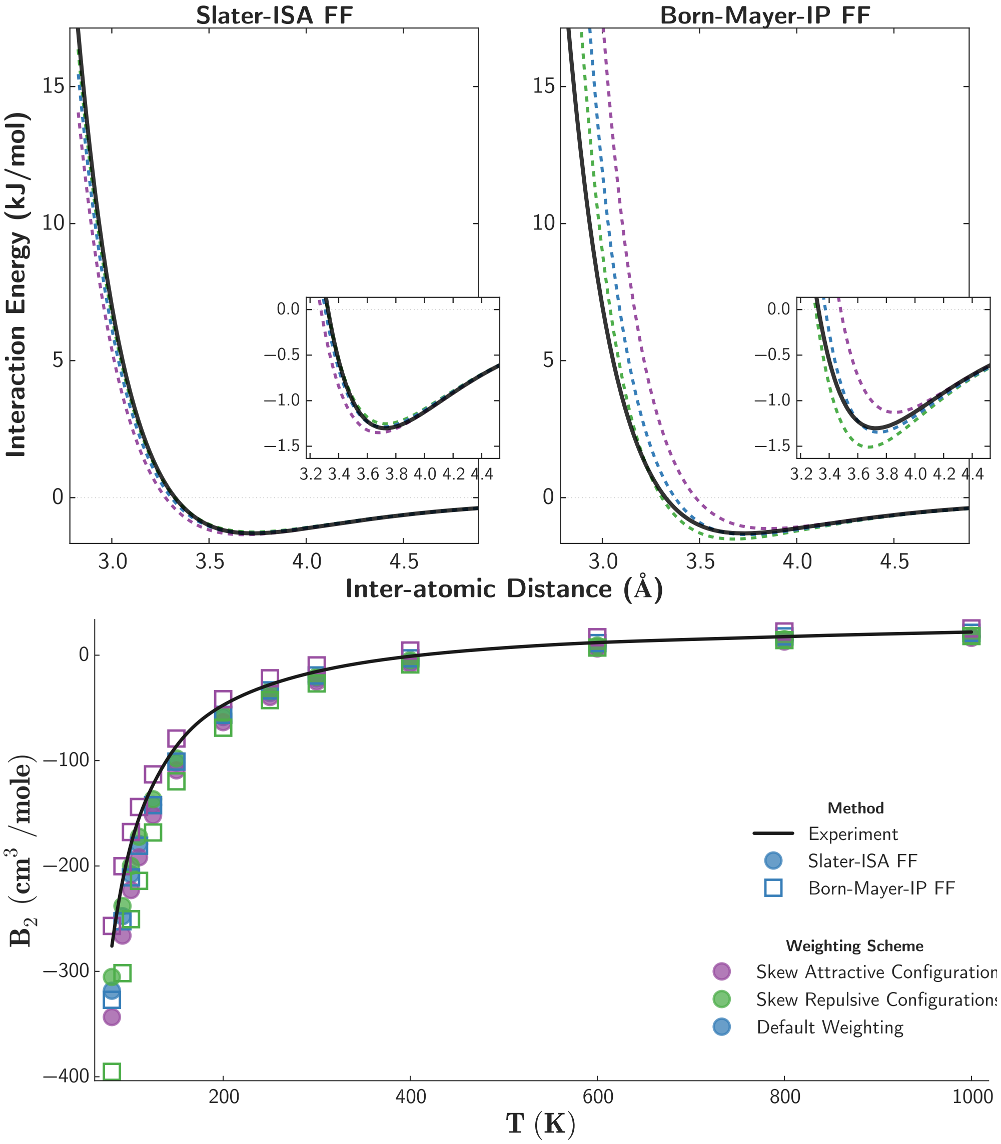


**Figure S10.** Comparison of the Slater-ISA FF and the Born-Mayer-IP FF in terms of sensitivity to the weighting function employed in parameter optimization for the Ar dimer. Three weighting functions, $\lambda = 0.5$ (purple), $\lambda = 2.0$ (blue), and $\lambda = 5.0$ (green) are shown, with higher $\lambda$ values indicating more weighting of repulsive configurations.
(top) Total interaction energies for the Slater-ISA FF (left) and the Born-Mayer-IP FF (right) indicating the accuracy of each force field with respect to DFT-SAPT (PBE0/AC) benchmark energies. DFT-SAPT energies are shown as black solid lines, force field fits with dotted lines. Colors for the different weighting functions is as above.
(bottom) Computed 2$^{\text{nd}}$ virial coefficients for argon. Data for the Slater-ISA FF and Born-Mayer-IP FF are depicted using open circles and shaded squares, respectively; coloration for the different weighting functions is as above. Experimental data from Dymond and Smith (black line) is also shown.

## S12 Parameter Robustness for Ethane; LJ FF results

Ethane parameters were tested for robustness by changing the weighting function as described in the main text. Optimized Slater-ISA FF $A_{ij}$ parameters are much less sensitive to the choice of weighting function compared to the LJ FF. As a result, the Slater-ISA FF shows decreased uncertainty when computing the $2^{\text{nd}}$ virial coefficient. Virial coefficients for the LJ FF, on the other hand, depend more strongly on the choice of weighting function.

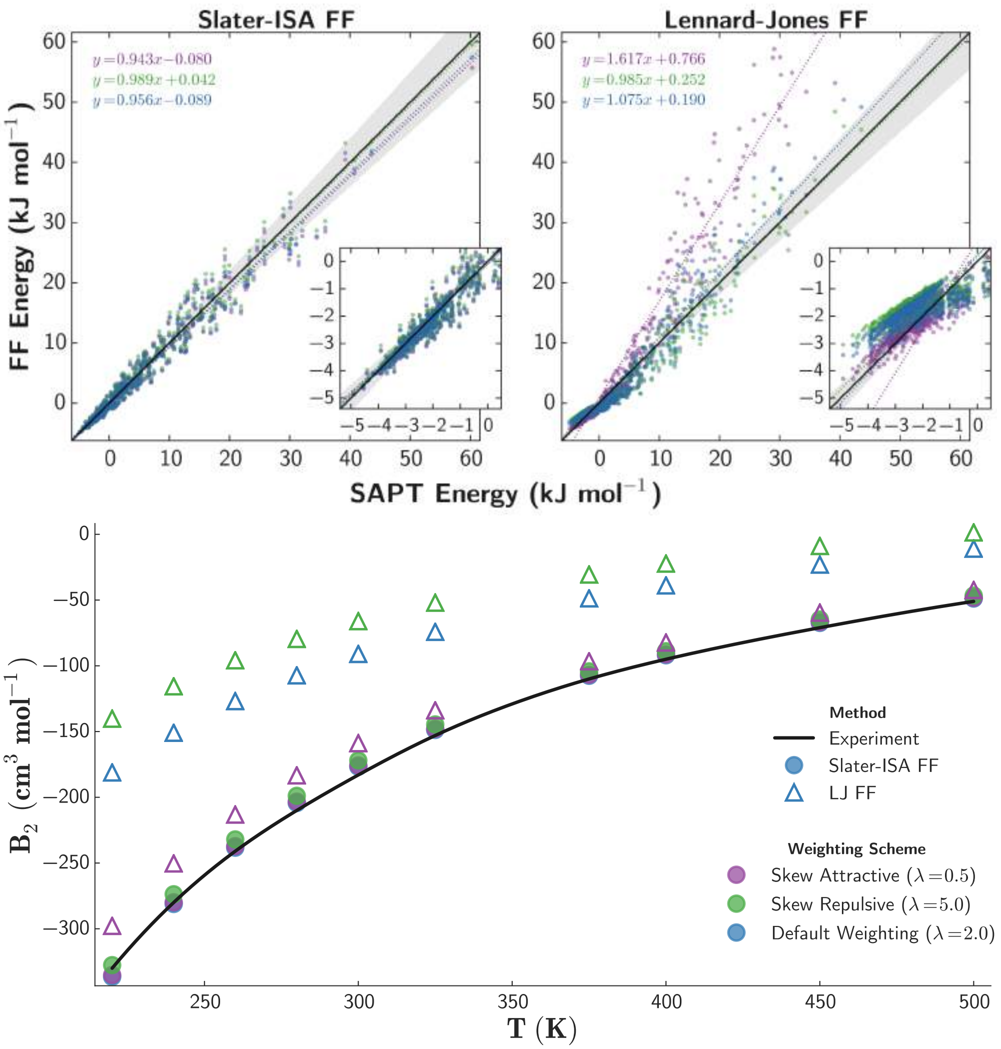


**Figure S11.** Comparison of the Slater-ISA FF and the LJ FF in terms of sensitivity to the weighting function employed in parameter optimization for the ethane dimer. Three weighting functions, $\lambda = 0.5$ (purple), $\lambda = 2.0$ (blue), and $\lambda = 5.0$ (green) are shown, with higher $\lambda$ values indicating more weighting of repulsive configurations.
(top) Total interaction energies for the Slater-ISA FF (left) and the LJ FF (right) indicating the accuracy of each force field with respect to DFT-SAPT (PBE0/AC) benchmark energies. The diagonal line (black) indicates perfect agreement between reference energies and each force field, while shaded grey areas represent points within ±10% agreement of the benchmark. To guide the eye, a line of best fit (dotted line) has been computed for each force field and for each weighting function.
(bottom) Computed 2$^{nd}$ virial coefficients for argon. Data for the Slater-ISA FF and the Born-Mayer-IP FF are depicted using open circles and shaded squares, respectively; coloration for the different weighting functions is as above. Experimental data from Dymond and Smith (black line) is also shown.

**Table S11.** Fitted values for Bij for a variety of element pairs. All values are given in atomic units, except for RMS errors, which are a unitless normalized overlap.

| $i$ | $j$ | $B_i$ | $B_j$ | $B_{ij}$ | RMSE | MAPE |
|---|---|---|---|---|---|---|
| H | He | 1.99946394 | 2.68859863 | 2.31740474 | 0.00044277657 | 0.882930 |
| H | Li | 1.99946394 | 1.25901971 | 1.59404909 | 0.00064319203 | 1.106033 |
| H | Be | 1.99946394 | 1.65554322 | 1.82052039 | 0.00012960395 | 0.217206 |
| H | B | 1.99946394 | 1.56191136 | 1.76768239 | 0.00022762336 | 0.498291 |
| H | C | 1.99946394 | 1.81946896 | 1.90742066 | 3.6383389e-05 | 0.074853 |
| H | N | 1.99946394 | 2.06711073 | 2.03302187 | 4.9406068e-06 | 0.009742 |
| H | O | 1.99946394 | 2.00091172 | 2.00019722 | 9.9506754e-08 | 0.000183 |
| H | F | 1.99946394 | 2.26322976 | 2.12730789 | 7.0666272e-05 | 0.137228 |
| H | Ne | 1.99946394 | 2.51791099 | 2.24270366 | 0.00026455338 | 0.578093 |
| H | Na | 1.99946394 | 1.22917354 | 1.57023314 | 0.00074952732 | 1.738728 |
| H | Mg | 1.99946394 | 1.49931366 | 1.73354253 | 0.0002881065 | 0.529739 |
| H | Al | 1.99946394 | 1.32657183 | 1.63349076 | 0.00053449852 | 0.976877 |
| H | Si | 1.99946394 | 1.54808130 | 1.75910683 | 0.00024917876 | 0.617006 |
| H | P | 1.99946394 | 1.75585679 | 1.87377325 | 6.8182489e-05 | 0.148197 |
| H | S | 1.99946394 | 1.74521745 | 1.86810662 | 7.4332699e-05 | 0.160880 |
| H | Cl | 1.99946394 | 1.95253790 | 1.97586738 | 2.5436846e-06 | 0.005705 |
| H | Ar | 1.99946394 | 2.15249556 | 2.07440522 | 2.5899665e-05 | 0.068500 |
| H | Br | 1.99946394 | 1.86365053 | 1.93033996 | 2.112332e-05 | 0.048965 |
| H | I | 1.99946394 | 1.75289066 | 1.87194355 | 7.1892596e-05 | 0.178949 |
| He | Li | 2.68859863 | 1.25901971 | 1.83579487 | 0.0020586815 | 4.802329 |
| He | Be | 2.68859863 | 1.65554322 | 2.10352673 | 0.0010603604 | 2.573450 |
| He | B | 2.68859863 | 1.56191136 | 2.03442611 | 0.00129508 | 3.918107 |
| He | C | 2.68859863 | 1.81946896 | 2.20238570 | 0.00075763278 | 2.262394 |
| He | N | 2.68859863 | 2.06711073 | 2.35237454 | 0.0003780889 | 1.127971 |
| He | O | 2.68859863 | 2.00091172 | 2.31393264 | 0.00046386026 | 1.314845 |
| He | F | 2.68859863 | 2.26322976 | 2.46423057 | 0.0001731239 | 0.522637 |
| He | Ne | 2.68859863 | 2.51791099 | 2.60133215 | 2.7253815e-05 | 0.094670 |
| He | Na | 2.68859863 | 1.22917354 | 1.79792813 | 0.0021797532 | 6.560866 |
| He | Mg | 2.68859863 | 1.49931366 | 1.99849093 | 0.0014277708 | 3.668547 |
| He | Al | 2.68859863 | 1.32657183 | 1.88040364 | 0.0018777097 | 4.668027 |
| He | Si | 2.68859863 | 1.54808130 | 2.02089719 | 0.001334628 | 4.489483 |
| He | P | 2.68859863 | 1.75585679 | 2.16119527 | 0.00087958401 | 2.730605 |
| He | S | 2.68859863 | 1.74521745 | 2.15451616 | 0.00090006465 | 2.778815 |
| He | Cl | 2.68859863 | 1.95253790 | 2.28271739 | 0.00054130424 | 1.785225 |
| He | Ar | 2.68859863 | 2.15249556 | 2.39953728 | 0.00028412395 | 1.122892 |
| He | Br | 2.68859863 | 1.86365053 | 2.22767127 | 0.00068597032 | 2.295912 |
| He | I | 2.68859863 | 1.75289066 | 2.15618545 | 0.0008917 | 3.122234 |
| Li | Be | 1.25901971 | 1.65554322 | 1.44552618 | 0.00021566494 | 0.459735 |
| Li | B | 1.25901971 | 1.56191136 | 1.40276036 | 0.00013669061 | 0.361720 |
| Li | C | 1.25901971 | 1.81946896 | 1.51465672 | 0.00042489929 | 1.056460 |
| Li | N | 1.25901971 | 2.06711073 | 1.61476325 | 0.00080816618 | 1.922263 |
| Li | O | 1.25901971 | 2.00091172 | 1.58945583 | 0.00069142836 | 1.593136 |

**Table S11 – continued from previous page**

| $i$ | $j$ | $B_i$ | $B_j$ | $B_{ij}$ | RMSE | MAPE |
|---|---|---|---|---|---|---|
| Li | F | 1.25901971 | 2.26322976 | 1.68919749 | 0.0011668895 | 2.718352 |
| Li | Ne | 1.25901971 | 2.51791099 | 1.77555429 | 0.0017026265 | 4.273871 |
| Li | Na | 1.25901971 | 1.22917354 | 1.24402068 | 1.5533688e-06 | 0.004373 |
| Li | Mg | 1.25901971 | 1.49931366 | 1.37457277 | 8.4735331e-05 | 0.195212 |
| Li | Al | 1.25901971 | 1.32657183 | 1.29242716 | 7.1019258e-06 | 0.016335 |
| Li | Si | 1.25901971 | 1.54808130 | 1.39618447 | 0.00012793291 | 0.374607 |
| Li | P | 1.25901971 | 1.75585679 | 1.48750641 | 0.00034426274 | 0.896554 |
| Li | S | 1.25901971 | 1.74521745 | 1.48302253 | 0.00033062213 | 0.858653 |
| Li | Cl | 1.25901971 | 1.95253790 | 1.56786800 | 0.00063028803 | 1.664314 |
| Li | Ar | 1.25901971 | 2.15249556 | 1.64158799 | 0.00099309611 | 2.932927 |
| Li | Br | 1.25901971 | 1.86365053 | 1.53172970 | 0.00049638053 | 1.350986 |
| Li | I | 1.25901971 | 1.75289066 | 1.48527643 | 0.00034799167 | 1.009017 |
| Be | B | 1.65554322 | 1.56191136 | 1.60804807 | 1.1972231e-05 | 0.031893 |
| Be | C | 1.65554322 | 1.81946896 | 1.73554580 | 3.3972736e-05 | 0.085743 |
| Be | N | 1.65554322 | 2.06711073 | 1.84956812 | 0.0001992019 | 0.484038 |
| Be | O | 1.65554322 | 2.00091172 | 1.82001716 | 0.00014155775 | 0.330806 |
| Be | F | 1.65554322 | 2.26322976 | 1.93457449 | 0.00041123838 | 0.983581 |
| Be | Ne | 1.65554322 | 2.51791099 | 2.03628351 | 0.00078343308 | 2.059895 |
| Be | Na | 1.65554322 | 1.22917354 | 1.42686604 | 0.00026737271 | 0.745777 |
| Be | Mg | 1.65554322 | 1.49931366 | 1.57563633 | 3.2478195e-05 | 0.074055 |
| Be | Al | 1.65554322 | 1.32657183 | 1.48286105 | 0.00014866739 | 0.335525 |
| Be | Si | 1.65554322 | 1.54808130 | 1.60086762 | 1.615263e-05 | 0.048036 |
| Be | P | 1.65554322 | 1.75585679 | 1.70494709 | 1.3101092e-05 | 0.034696 |
| Be | S | 1.65554322 | 1.74521745 | 1.69977980 | 1.0504303e-05 | 0.027715 |
| Be | Cl | 1.65554322 | 1.95253790 | 1.79750301 | 0.00010922498 | 0.297117 |
| Be | Ar | 1.65554322 | 2.15249556 | 1.88512628 | 0.00029576275 | 0.923403 |
| Be | Br | 1.65554322 | 1.86365053 | 1.75630627 | 5.5219463e-05 | 0.154638 |
| Be | I | 1.65554322 | 1.75289066 | 1.70346914 | 1.2636043e-05 | 0.037713 |
| B | C | 1.56191136 | 1.81946896 | 1.68526246 | 8.896852e-05 | 0.279460 |
| B | N | 1.56191136 | 2.06711073 | 1.79465183 | 0.00031660316 | 0.962841 |
| B | O | 1.56191136 | 2.00091172 | 1.76649990 | 0.00024246047 | 0.712022 |
| B | F | 1.56191136 | 2.26322976 | 1.87554766 | 0.00057369687 | 1.719903 |
| B | Ne | 1.56191136 | 2.51791099 | 1.97105959 | 0.00099084843 | 3.222525 |
| B | Na | 1.56191136 | 1.22917354 | 1.38509763 | 0.00017473338 | 0.590078 |
| B | Mg | 1.56191136 | 1.49931366 | 1.53029477 | 5.6807294e-06 | 0.016154 |
| B | Al | 1.56191136 | 1.32657183 | 1.43954012 | 8.2359665e-05 | 0.230371 |
| B | Si | 1.56191136 | 1.54808130 | 1.55498504 | 3.4970147e-07 | 0.001260 |
| B | P | 1.56191136 | 1.75585679 | 1.65571982 | 5.1764703e-05 | 0.169673 |
| B | S | 1.56191136 | 1.74521745 | 1.65073751 | 4.6359978e-05 | 0.151426 |
| B | Cl | 1.56191136 | 1.95253790 | 1.74462228 | 0.00019882685 | 0.668654 |
| B | Ar | 1.56191136 | 2.15249556 | 1.82774537 | 0.00043254436 | 1.644894 |
| B | Br | 1.56191136 | 1.86365053 | 1.70507656 | 0.00012232055 | 0.422076 |
| B | I | 1.56191136 | 1.75289066 | 1.65418604 | 5.1089297e-05 | 0.186574 |
| C | N | 1.81946896 | 2.06711073 | 1.93878424 | 7.2588349e-05 | 0.213967 |
| C | O | 1.81946896 | 2.00091172 | 1.90779431 | 3.9381872e-05 | 0.111509 |

**Table S11 – continued from previous page**

| $i$ | $j$ | $B_i$ | $B_j$ | $B_{ij}$ | RMSE | MAPE |
|---|---|---|---|---|---|---|
| C | F | 1.81946896 | 2.26322976 | 2.02729827 | 0.00022128603 | 0.646349 |
| C | Ne | 1.81946896 | 2.51791099 | 2.13356824 | 0.00051712548 | 1.665041 |
| C | Na | 1.81946896 | 1.22917354 | 1.49359005 | 0.00049650546 | 1.590315 |
| C | Mg | 1.81946896 | 1.49931366 | 1.65145683 | 0.00013523926 | 0.364498 |
| C | Al | 1.81946896 | 1.32657183 | 1.55375705 | 0.00032909645 | 0.868090 |
| C | Si | 1.81946896 | 1.54808130 | 1.67745495 | 0.00010070423 | 0.351275 |
| C | P | 1.81946896 | 1.75585679 | 1.78734889 | 5.2847945e-06 | 0.016690 |
| C | S | 1.81946896 | 1.74521745 | 1.78191233 | 7.1848878e-06 | 0.022600 |
| C | Cl | 1.81946896 | 1.95253790 | 1.88462580 | 2.1955555e-05 | 0.071858 |
| C | Ar | 1.81946896 | 2.15249556 | 1.97704725 | 0.0001323859 | 0.499304 |
| C | Br | 1.81946896 | 1.86365053 | 1.84141110 | 2.5492317e-06 | 0.008538 |
| C | I | 1.81946896 | 1.75289066 | 1.78581710 | 5.8824253e-06 | 0.020847 |
| N | O | 2.06711073 | 2.00091172 | 2.03371451 | 5.041231e-06 | 0.013929 |
| N | F | 2.06711073 | 2.26322976 | 2.16254689 | 4.15042e-05 | 0.119485 |
| N | Ne | 2.06711073 | 2.51791099 | 2.27840189 | 0.00020910088 | 0.673215 |
| N | Na | 2.06711073 | 1.22917354 | 1.58958212 | 0.00090815621 | 2.796799 |
| N | Mg | 2.06711073 | 1.49931366 | 1.75954426 | 0.00039310972 | 1.019328 |
| N | Al | 2.06711073 | 1.32657183 | 1.65570661 | 0.00068105488 | 1.722447 |
| N | Si | 2.06711073 | 1.54808130 | 1.78559923 | 0.00033982883 | 1.150687 |
| N | P | 2.06711073 | 1.75585679 | 1.90415582 | 0.00011669305 | 0.359120 |
| N | S | 2.06711073 | 1.74521745 | 1.89832775 | 0.00012494822 | 0.382742 |
| N | Cl | 2.06711073 | 1.95253790 | 2.00885032 | 1.5404889e-05 | 0.049510 |
| N | Ar | 2.06711073 | 2.15249556 | 2.10924579 | 8.3837241e-06 | 0.031515 |
| N | Br | 2.06711073 | 1.86365053 | 1.96222048 | 4.938888e-05 | 0.162281 |
| N | I | 2.06711073 | 1.75289066 | 1.90214169 | 0.00012093134 | 0.419448 |
| O | F | 2.00091172 | 2.26322976 | 2.12742019 | 7.4513608e-05 | 0.204667 |
| O | Ne | 2.00091172 | 2.51791099 | 2.24105845 | 0.00027602296 | 0.845765 |
| O | Na | 2.00091172 | 1.22917354 | 1.56546880 | 0.00078625246 | 2.354990 |
| O | Mg | 2.00091172 | 1.49931366 | 1.73176044 | 0.00031061975 | 0.777382 |
| O | Al | 2.00091172 | 1.32657183 | 1.62980355 | 0.00057319586 | 1.403523 |
| O | Si | 2.00091172 | 1.54808130 | 1.75782981 | 0.00026287602 | 0.860753 |
| O | P | 2.00091172 | 1.75585679 | 1.87387688 | 7.3175089e-05 | 0.216650 |
| O | S | 2.00091172 | 1.74521745 | 1.86815729 | 7.9760452e-05 | 0.235090 |
| O | Cl | 2.00091172 | 1.95253790 | 1.97655937 | 2.8387158e-06 | 0.008742 |
| O | Ar | 2.00091172 | 2.15249556 | 2.07494432 | 2.6479263e-05 | 0.095246 |
| O | Br | 2.00091172 | 1.86365053 | 1.93085797 | 2.2760392e-05 | 0.071837 |
| O | I | 2.00091172 | 1.75289066 | 1.87203787 | 7.6356395e-05 | 0.255064 |
| F | Ne | 2.26322976 | 2.51791099 | 2.38617019 | 6.4967098e-05 | 0.211473 |
| F | Na | 2.26322976 | 1.22917354 | 1.66029149 | 0.0012830926 | 3.875179 |
| F | Mg | 2.26322976 | 1.49931366 | 1.83986590 | 0.00066962961 | 1.706670 |
| F | Al | 2.26322976 | 1.32657183 | 1.73140874 | 0.0010196712 | 2.528620 |
| F | Si | 2.26322976 | 1.54808130 | 1.86526151 | 0.00060490347 | 2.020578 |
| F | P | 2.26322976 | 1.75585679 | 1.99065290 | 0.00029360355 | 0.894671 |
| F | S | 2.26322976 | 1.74521745 | 1.98453998 | 0.00030630021 | 0.928727 |
| F | Cl | 2.26322976 | 1.95253790 | 2.10087150 | 0.00010755539 | 0.344316 |

**Table S11 – continued from previous page**

| $i$ | $j$ | $B_i$ | $B_j$ | $B_{ij}$ | RMSE | MAPE |
|---|---|---|---|---|---|---|
| F | Ar | 2.26322976 | 2.15249556 | 2.20694293 | 1.3485721e-05 | 0.050987 |
| F | Br | 2.26322976 | 1.86365053 | 2.05158173 | 0.00018081195 | 0.590554 |
| F | I | 2.26322976 | 1.75289066 | 1.98794200 | 0.00030142935 | 1.036990 |
| Ne | Na | 2.51791099 | 1.22917354 | 1.74146757 | 0.0018171227 | 5.842510 |
| Ne | Mg | 2.51791099 | 1.49931366 | 1.93474540 | 0.0011134419 | 3.086201 |
| Ne | Al | 2.51791099 | 1.32657183 | 1.81962923 | 0.001531155 | 4.095464 |
| Ne | Si | 2.51791099 | 1.54808130 | 1.95888870 | 0.0010266525 | 3.702217 |
| Ne | P | 2.51791099 | 1.75585679 | 2.09400464 | 0.00062146304 | 2.076964 |
| Ne | S | 2.51791099 | 1.74521745 | 2.08750459 | 0.00063928574 | 2.124924 |
| Ne | Cl | 2.51791099 | 1.95253790 | 2.21174754 | 0.00033656173 | 1.193911 |
| Ne | Ar | 2.51791099 | 2.15249556 | 2.32497739 | 0.00013843693 | 0.584890 |
| Ne | Br | 2.51791099 | 1.86365053 | 2.15873868 | 0.0004557 | 1.639505 |
| Ne | I | 2.51791099 | 1.75289066 | 2.09004196 | 0.00063134274 | 2.372214 |
| Na | Mg | 1.22917354 | 1.49931366 | 1.35766104 | 0.00011473889 | 0.341738 |
| Na | Al | 1.22917354 | 1.32657183 | 1.27699602 | 1.5803838e-05 | 0.046721 |
| Na | Si | 1.22917354 | 1.54808130 | 1.37861851 | 0.00016394224 | 0.606312 |
| Na | P | 1.22917354 | 1.75585679 | 1.46734689 | 0.00040724885 | 1.358887 |
| Na | S | 1.22917354 | 1.74521745 | 1.46301699 | 0.00039233117 | 1.305796 |
| Na | Cl | 1.22917354 | 1.95253790 | 1.54462666 | 0.00071489747 | 2.415615 |
| Na | Ar | 1.22917354 | 2.15249556 | 1.61475657 | 0.0010865392 | 4.048855 |
| Na | Br | 1.22917354 | 1.86365053 | 1.50991318 | 0.00057095415 | 1.982122 |
| Na | I | 1.22917354 | 1.75289066 | 1.46507909 | 0.00040898615 | 1.502211 |
| Mg | Al | 1.49931366 | 1.32657183 | 1.41054381 | 4.3759475e-05 | 0.106460 |
| Mg | Si | 1.49931366 | 1.54808130 | 1.52349731 | 3.5595022e-06 | 0.011234 |
| Mg | P | 1.49931366 | 1.75585679 | 1.62233525 | 8.9250076e-05 | 0.251892 |
| Mg | S | 1.49931366 | 1.74521745 | 1.61744114 | 8.2197924e-05 | 0.231214 |
| Mg | Cl | 1.49931366 | 1.95253790 | 1.70986111 | 0.00026403315 | 0.761802 |
| Mg | Ar | 1.49931366 | 2.15249556 | 1.79169870 | 0.00052474149 | 1.715332 |
| Mg | Br | 1.49931366 | 1.86365053 | 1.67083027 | 0.00017608345 | 0.522795 |
| Mg | I | 1.49931366 | 1.75289066 | 1.62071071 | 8.9123446e-05 | 0.281480 |
| Al | Si | 1.32657183 | 1.54808130 | 1.43295795 | 7.4878405e-05 | 0.231698 |
| Al | P | 1.32657183 | 1.75585679 | 1.52615042 | 0.00025709446 | 0.709802 |
| Al | S | 1.32657183 | 1.74521745 | 1.52156219 | 0.00024519155 | 0.674974 |
| Al | Cl | 1.32657183 | 1.95253790 | 1.60826232 | 0.00051441718 | 1.443233 |
| Al | Ar | 1.32657183 | 2.15249556 | 1.68396084 | 0.0008502512 | 2.673094 |
| Al | Br | 1.32657183 | 1.86365053 | 1.57145555 | 0.00039199648 | 1.132597 |
| Al | I | 1.32657183 | 1.75289066 | 1.52414100 | 0.00025909364 | 0.796534 |
| Si | P | 1.54808130 | 1.75585679 | 1.64816385 | 6.0537472e-05 | 0.219836 |
| Si | S | 1.54808130 | 1.74521745 | 1.64322319 | 5.4646042e-05 | 0.197756 |
| Si | Cl | 1.54808130 | 1.95253790 | 1.73616531 | 0.00021653004 | 0.806893 |
| Si | Ar | 1.54808130 | 2.15249556 | 1.81809419 | 0.00045725342 | 1.916727 |
| Si | Br | 1.54808130 | 1.86365053 | 1.69704848 | 0.00013598439 | 0.519161 |
| Si | I | 1.54808130 | 1.75289066 | 1.64662155 | 5.971014e-05 | 0.240522 |
| P | S | 1.75585679 | 1.74521745 | 1.75053498 | 2.2383111e-07 | 0.000726 |
| P | Cl | 1.75585679 | 1.95253790 | 1.85109487 | 4.8767404e-05 | 0.166222 |

Table S11 – continued from previous page

| $i$ | $j$ | $B_i$ | $B_j$ | $B_{ij}$ | RMSE | MAPE |
|---|---|---|---|---|---|---|
| P | Ar | 1.75585679 | 2.15249556 | 1.94118289 | 0.00019034099 | 0.743408 |
| P | Br | 1.75585679 | 1.86365053 | 1.80880477 | 1.5089803e-05 | 0.052666 |
| P | I | 1.75585679 | 1.75289066 | 1.75438024 | 8.3311914e-08 | 0.000297 |
| S | Cl | 1.74521745 | 1.95253790 | 1.84542979 | 5.4259063e-05 | 0.184109 |
| S | Ar | 1.74521745 | 2.15249556 | 1.93516069 | 0.00020092813 | 0.780785 |
| S | Br | 1.74521745 | 1.86365053 | 1.80328668 | 1.8231579e-05 | 0.063360 |
| S | I | 1.74521745 | 1.75289066 | 1.74905593 | 1.5042953e-07 | 0.000542 |
| Cl | Ar | 1.95253790 | 2.15249556 | 2.04925011 | 4.7026489e-05 | 0.193758 |
| Cl | Br | 1.95253790 | 1.86365053 | 1.90746100 | 9.8799774e-06 | 0.035850 |
| Cl | I | 1.95253790 | 1.75289066 | 1.84935929 | 5.0999292e-05 | 0.194814 |
| Ar | Br | 2.15249556 | 1.86365053 | 2.00111347 | 9.9755127e-05 | 0.417023 |
| Ar | I | 2.15249556 | 1.75289066 | 1.93889388 | 0.00019497498 | 0.849907 |
| Br | I | 1.86365053 | 1.75289066 | 1.80721936 | 1.6163908e-05 | 0.063089 |

# References


[1] Yu, K.; McDaniel, J. G.; Schmidt, J. R. *J. Phys. Chem. B* **2011**, *115*, 10054–10063.

[2] Waldman, M.; Hagler, A. T. *J. Comput. Chem.* **1993**, *14*, 1077–1084.

[3] Rosen, N. *Phys. Rev. Lett.* **1931**, *38*, 255–276.

[4] Tai, H. *Phys. Rev. A* **1986**, *33*, 3657–3666.

[5] Stone, A. J. *The Theory of Intermolecular Forces*, 2nd ed.; OUP Oxford, 2013.

[6] Dymond, J. H.; Smith, E. B. *The Virial Coefficients of Pure Gases and Mixtures*, 2nd ed.; Clarendon Press: Berlin Heidelberg, 1980.
